# Supplementary material for: A data-centric approach for assessing progress of Graph Neural Networks
Source: arXiv:2406.12439 source file (2024-06-18)
Supplement: Supplementary file 1 [file appendix.tex]

\section{}
\mpara{Organization.} We propose $3$ new biological datsets in \ref{sec:new_bio} and explain the construction details of the biological datasets in \ref{BioConstruction}. Furthermore, in Section \ref{sec:parameterstudy}, we study the parameters of the graph generator and demonstrate how we generate the synthetic datasets with varying label homophily. We also summarize the characteristics of the generated synthetic graphs that were used in Section \ref{experiments} for the varying homophily and feature quality experiments. In Section \ref{hyperpara}, we summarize the hyperparameters of the models we used in this work. In Section \ref{Experiment Results}, we provide the full original experiment results on all datasets reported in Micro- and Macro- F1, AUROC, and Average Precision score with the standard deviation of the $3$ random splits if the dataset is not pre-splitted. Note that for higher precision, the scores are provided in percentages. Last but not least, we provide the motivation for using Average Precision in the main paper in Section \ref{MetricDisscusion}.

\subsection{ New biological interaction datasets}
\label{sec:new_bio}
Motivated by the natural applicability of the multi-label classification task in various biological datasets and to improve the representativeness of available datasets, we collect three real-world biological datasets corresponding to different multi-label classification problems: the \pcg dataset for the protein phenotype prediction, the \humloc, and \eukloc datasets for the human and eukaryote protein subcellular location prediction tasks, respectively. On each dataset, we build a graph in which each protein is modeled as a node. The node label is the corresponding protein's label. An edge represents a known interaction between two proteins retrieved from a public database. The detailed pre-processing steps and the original data sources are discussed in Appendix \ref{phenotypeDataDes},~\ref{humLocDes}, and~\ref{eukLocDes}. Table~\ref{tab:newdataset} presents an overview of the three datasets' characteristics.
\label{sec:biologicaldatasets}

\begin{table}[!h] 

\setlength{\tabcolsep}{3pt}
 \caption{Statistics for new datasets. The column notations are the same as in Table \ref{tab:dataset}.  }
\small
\centering
 \begin{tabular}{lccccccccccccc}
\toprule

\textsc{Dataset}             &  $|\mathcal{V}|$  & $|\mathcal{E}|$ &  $|\mathcal{F}|$    &  $clus$  &$r_{homo}$ & $C$ &$\ell_{med}$& $\ell_{mean}$  & $\ell_{max}$& $25$\% & $50$\% & $75$\%\\
  
\midrule
 \pcg   &3K   &37k   &32&0.34&0.17&15&1&1.93&12&1&1&2\\
 \humloc  &3.10k   &18K   &32&0.13&0.42&14&1&1.19&4&1&1&1\\
 \eukloc  &7.70K  &13K   &32&0.14&0.46&22&1&1.15&4&1&1&1\\
 \hline
 \end{tabular}
 \label{tab:newdataset}
\end{table}

\begin{wrapfigure}{r}{0.4\textwidth}
\includegraphics[width=1.0\linewidth]{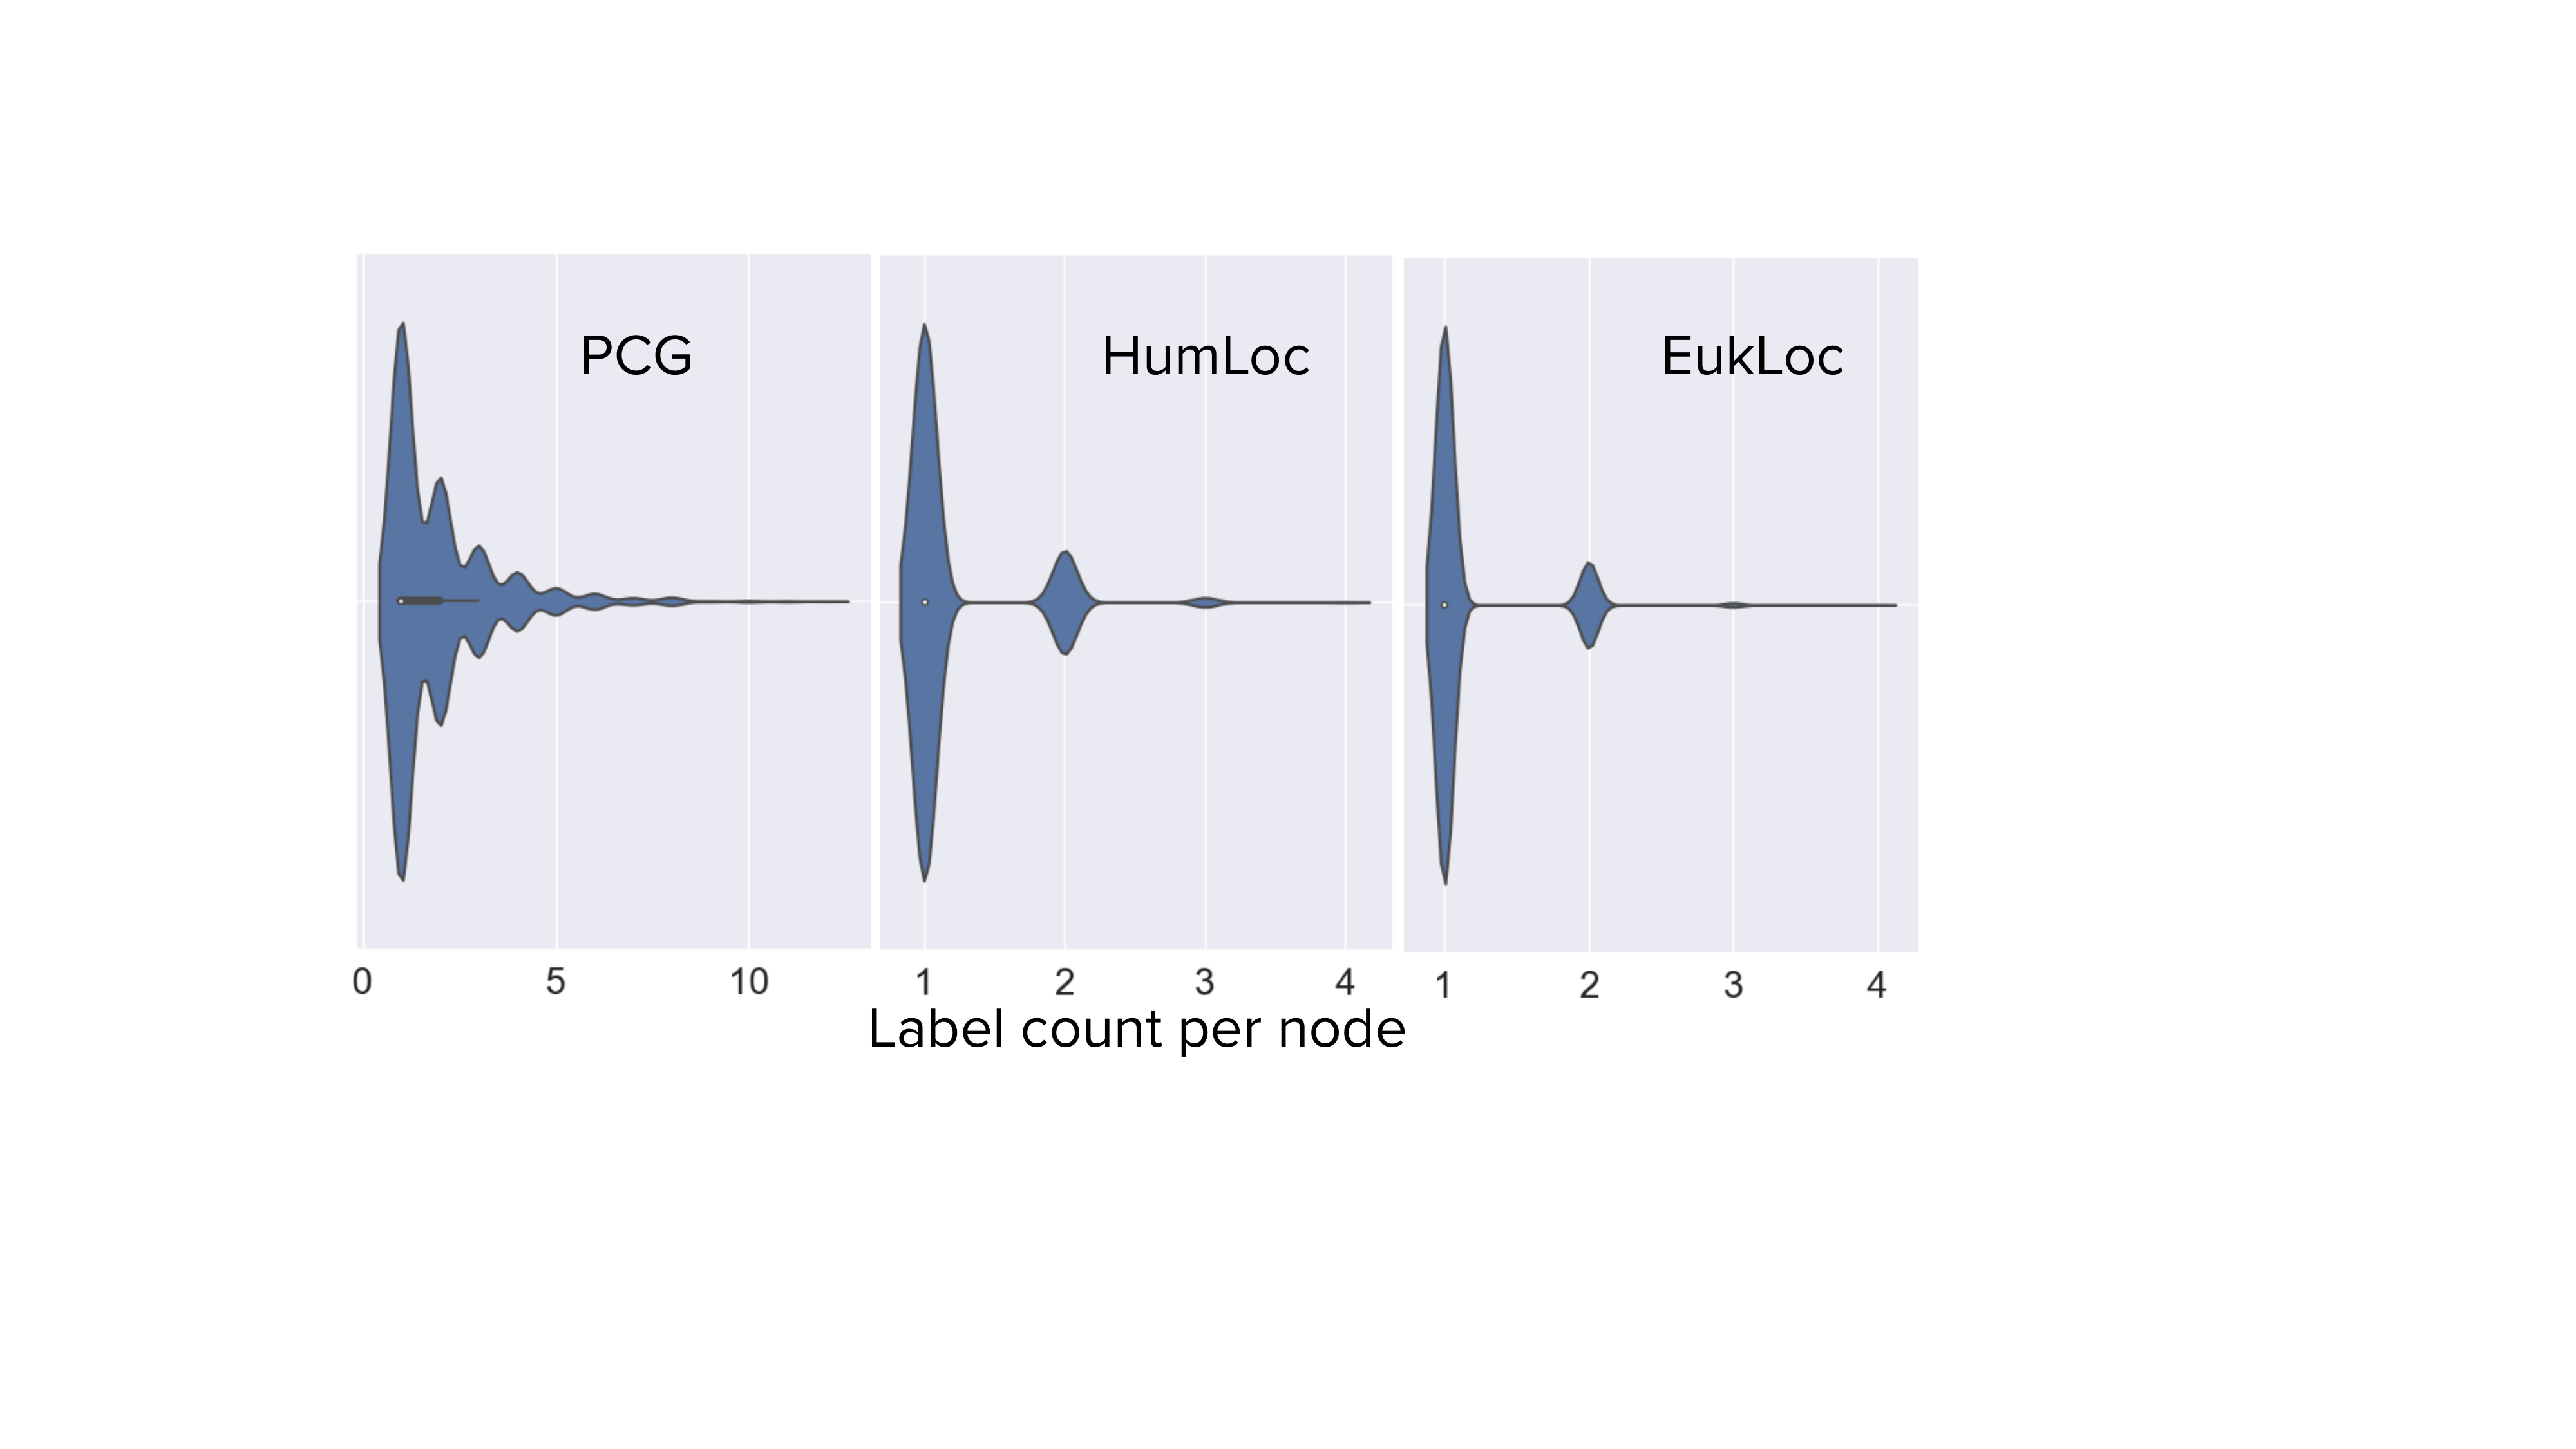} 
\caption{Label distributions in biological datasets. The majority of the nodes in all datasets have one label.}
\label{fig:labeldistbio}
\end{wrapfigure}

While all the existing datasets had very low homophily, \humloc, and \eukloc show higher homophily. Moreover, these datasets improve the representativeness in terms of varying graph structure (reflected in computed clustering coefficient) and in node, edge, and feature sizes. On the downside, these datasets also show a similar low multi-label character, with the majority of nodes in these datasets still having a single label. Among the three datasets, \pcg shows a bit more balanced label distribution (see Figure \ref{fig:labeldistbio}) as compared to the other two. Figure \ref{fig:ccns_bio} provides the cross-class neighborhood similarity scores. All three datasets show different patterns according to CCNS measure which is desirable to analyse the differences in method's performance.
While in PCG we see an overall high scores for CCNS, the difference in inter- and intra- class similarities is not prominent.
\humloc shows a slightly more contrasting intra- and inter-class neighborhood similarity. \eukloc, on the other hand, show very small neighborhood label similarities for nodes of same or different classes.
\begin{figure}[h!]
     \centering
     \begin{subfigure}[b]{0.3\textwidth}
         \centering
         \includegraphics[width=\textwidth]{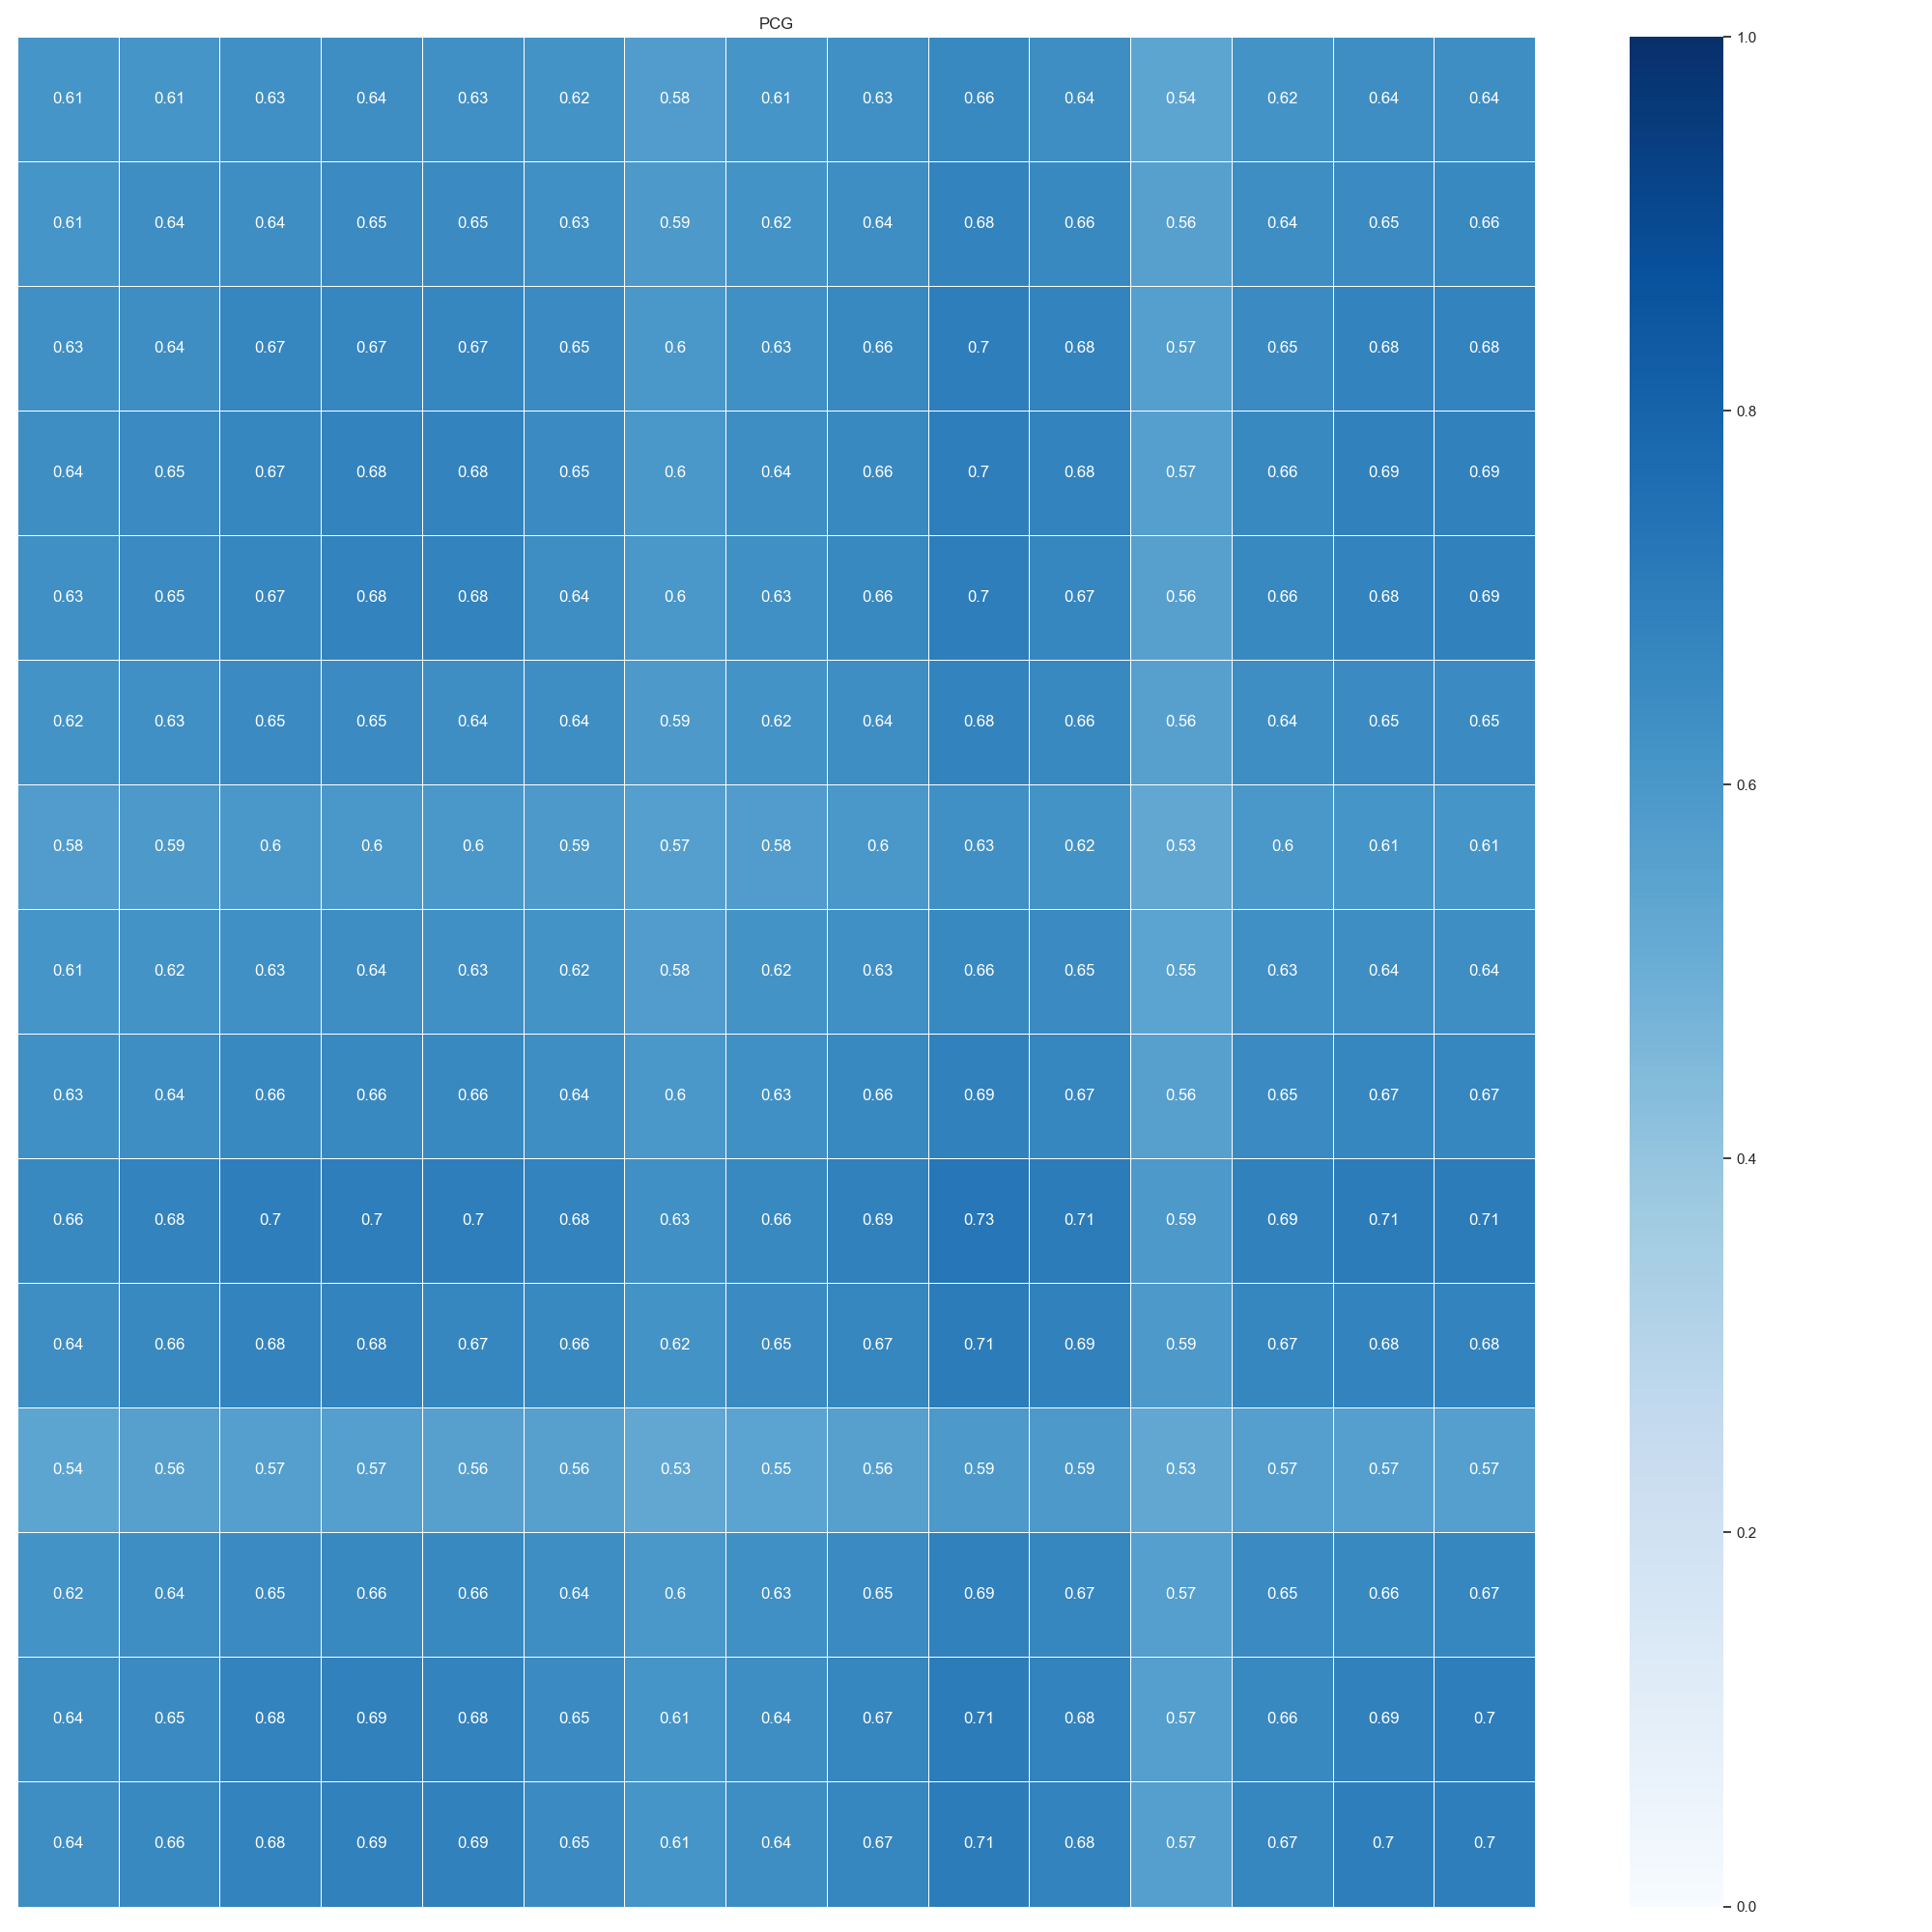}
         \caption{Cross class Neighborhood Similarity in \pcg}
         \label{fig:ccns_pcg}
     \end{subfigure}
     \hfill
     \begin{subfigure}[b]{0.3\textwidth}
         \centering
         \includegraphics[width=\textwidth]{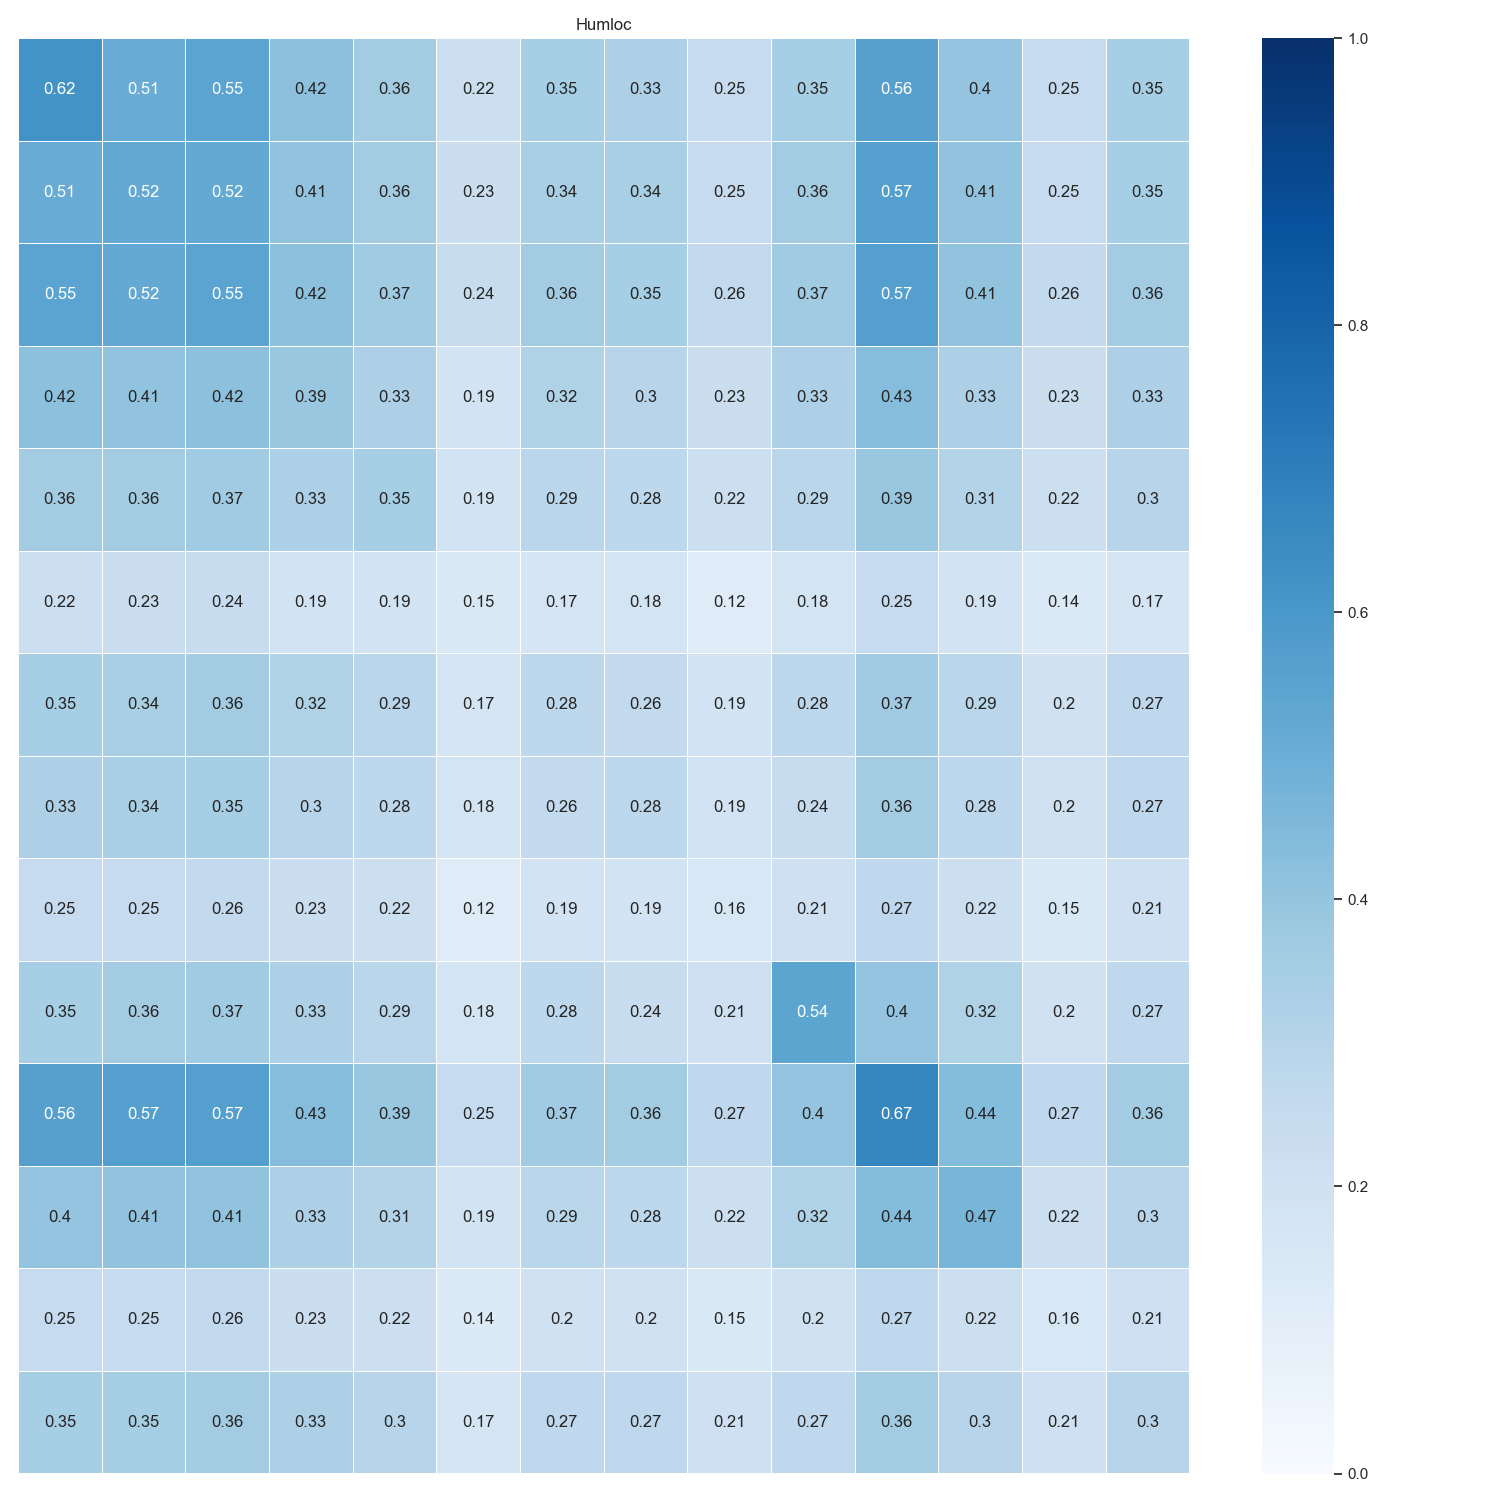}
         \caption{Cross class Neighborhood Similarity in \humloc}
         \label{fig:ccns_humloc}
     \end{subfigure}
     \hfill
     \begin{subfigure}[b]{0.3\textwidth}
         \centering
         \includegraphics[width=\textwidth]{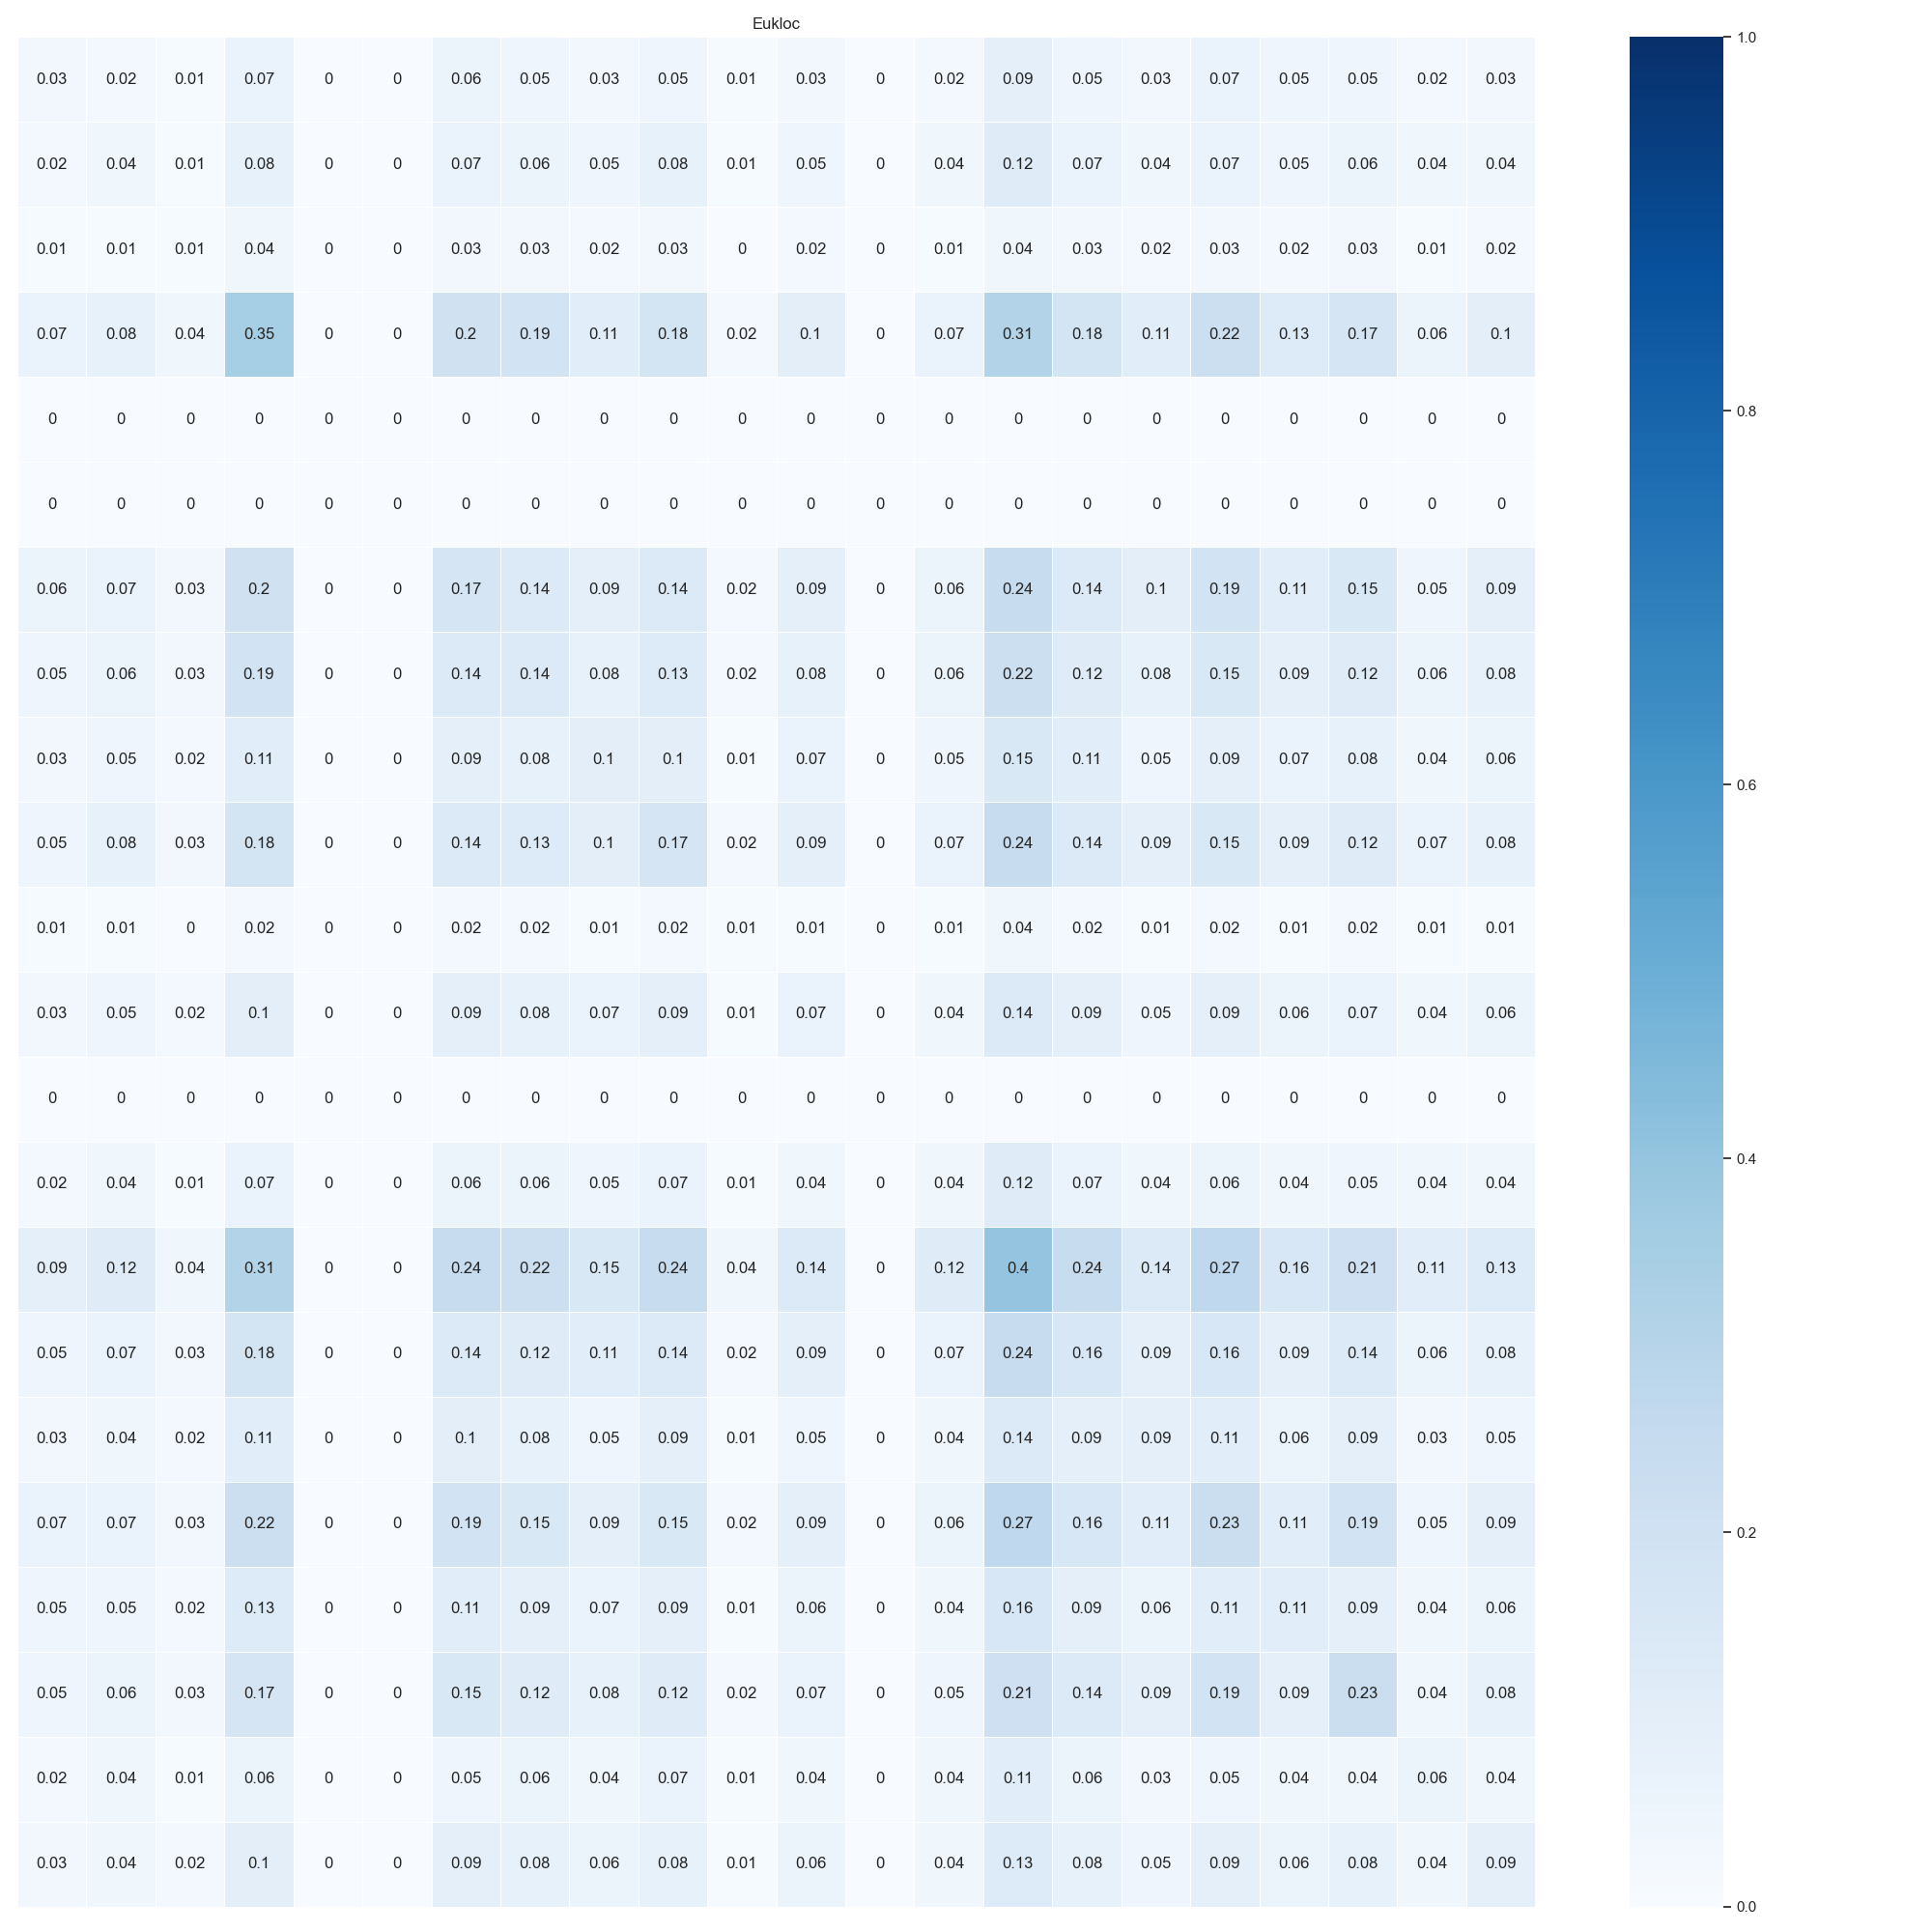}
         \caption{Cross class Neighborhood Similarity in \eukloc}
         \label{fig:ccns_eukloc}
     \end{subfigure}
        \caption{Cross class Neighborhood Similarity in real-world datasets and proposed biological datasets}
        \label{fig:ccns_bio}
\end{figure}

\subsection{Biological Dataset Construction}
\label{BioConstruction}
\subsubsection{The Protein phenotype prediction dataset.}
\label{phenotypeDataDes}
A phenotype is any observable characteristic or trait of a disease. Identifying the phenotypes associated with a particular protein could help in clinical diagnostics or finding possible drug targets. 

To construct the phenotype prediction dataset, we first retrieve the experimentally validated protein-phenotype associations from the DisGeNET~\citep{pinero2020disgenet} database. We then (i) retain only those protein associations that are marked as ``phenotype'', (ii) match each disease to its first-level category in the MESH ontology~\citep{bhattacharya2011mesh}, and (iii) remove any (phenotype) label with less than 100 associated proteins. 
To construct the edges, we acquire the protein functional interaction network from \citep{wu2010human} (version 2020). We then (i) model each protein as a node in the graph, (ii) retain only the protein-protein interactions between the proteins that have the phenotype labels available, and (iii) remove any isolated nodes from the constructed graph. In the end, our dataset consists of $3,233$ proteins and $37,351$ edges. The node features are the 32-dimensional sequence-based embeddings retrieved from ~\citep{uniprot2015uniprot} and \citep{yang2020prediction}.

\subsubsection{The human protein subcellular location prediction dataset (\humloc).}
\label{humLocDes}
Proteins might exist at or move between different subcellular locations. Predicting protein subcellular locations can aid the identification of drug targets\footnote{\href{https://en.wikipedia.org/wiki/Protein_subcellular_localization_prediction}{\url{https://en.wikipedia.org/wiki/Protein_subcellular_localization_prediction}}}.
We retrieve the human protein subcellular location data from \citep{shen2007hum} which contains $3,106$ proteins. Each protein can have one to several labels in $14$ possible locations. We then generate the graph multi-label node classification data as follows:
\begin{itemize}[leftmargin=*]
    \item We model each protein as a node in the graph. We retrieve the corresponding protein sequences from Uniprot \citep{uniprot2015uniprot}. We obtain the corresponding $32$-dimensional node feature representation by feeding them to a  pre-trained model~\citep{yang2020prediction} on protein sequences.
    \item Each node's label is the one-hot encoding (i.e., $14$ dimensions) generated from its sub-cellular information. Each value in the label vector represents one sub-cellular location. A value of $1$ indicates the corresponding protein exists at the respective location and $0$ means otherwise.
   
    \item The edge information is generated from the protein-protein interactions retrieved from the IntAct~\citep{kerrien2012intact} database. There exists a connection between two nodes in the graph if there exists an interaction between the corresponding proteins in IntAct. For each pair of proteins, more than one interaction of different types might exist. Therefore, we assign each edge a label. The edge label is modeled as a 21-dimensional vector where each value in the vector represents the confidence score for a particular connection type.
\end{itemize}
In the end, the \humloc dataset consists of 3,106 nodes and 18,496 edges. Each node can have one to several labels in the 14 possible locations.
Among the 3,106 different proteins, 2,580 of them belong only to 1 location; 480 of them belong to 2 locations; 43 of them belong to 3 locations and 3 of them belong to 4 locations. Both the accession numbers and sequences are given. None of the proteins has more than 25\% sequence identity to any other in the same subset (subcellular location). For a more detailed description of the original dataset, we refer the readers to \citep{shen2007hum}.

\subsubsection{The eukaryote protein subcellular location prediction dataset (\eukloc).}
\label{eukLocDes}
We retrieve the eukaryote protein subcellular location multi-label data from \citep{chou2007euk}. We then employ the same data sources and pre-processing strategy as described for the \humloc dataset to generate the multi-label node classification dataset for eukaryote protein subcellular location prediction. In the end, the final pre-processed data contains 7,766 proteins (nodes) and 13,818 connections(edges). Each protein(node) can receive one to several labels in 22 possible locations.

\subsection{Parameter Study of the Graph Generator Model}
\label{sec:parameterstudy}
\begin{figure}[h!]
    \centering
    \includegraphics[width=1\textwidth]{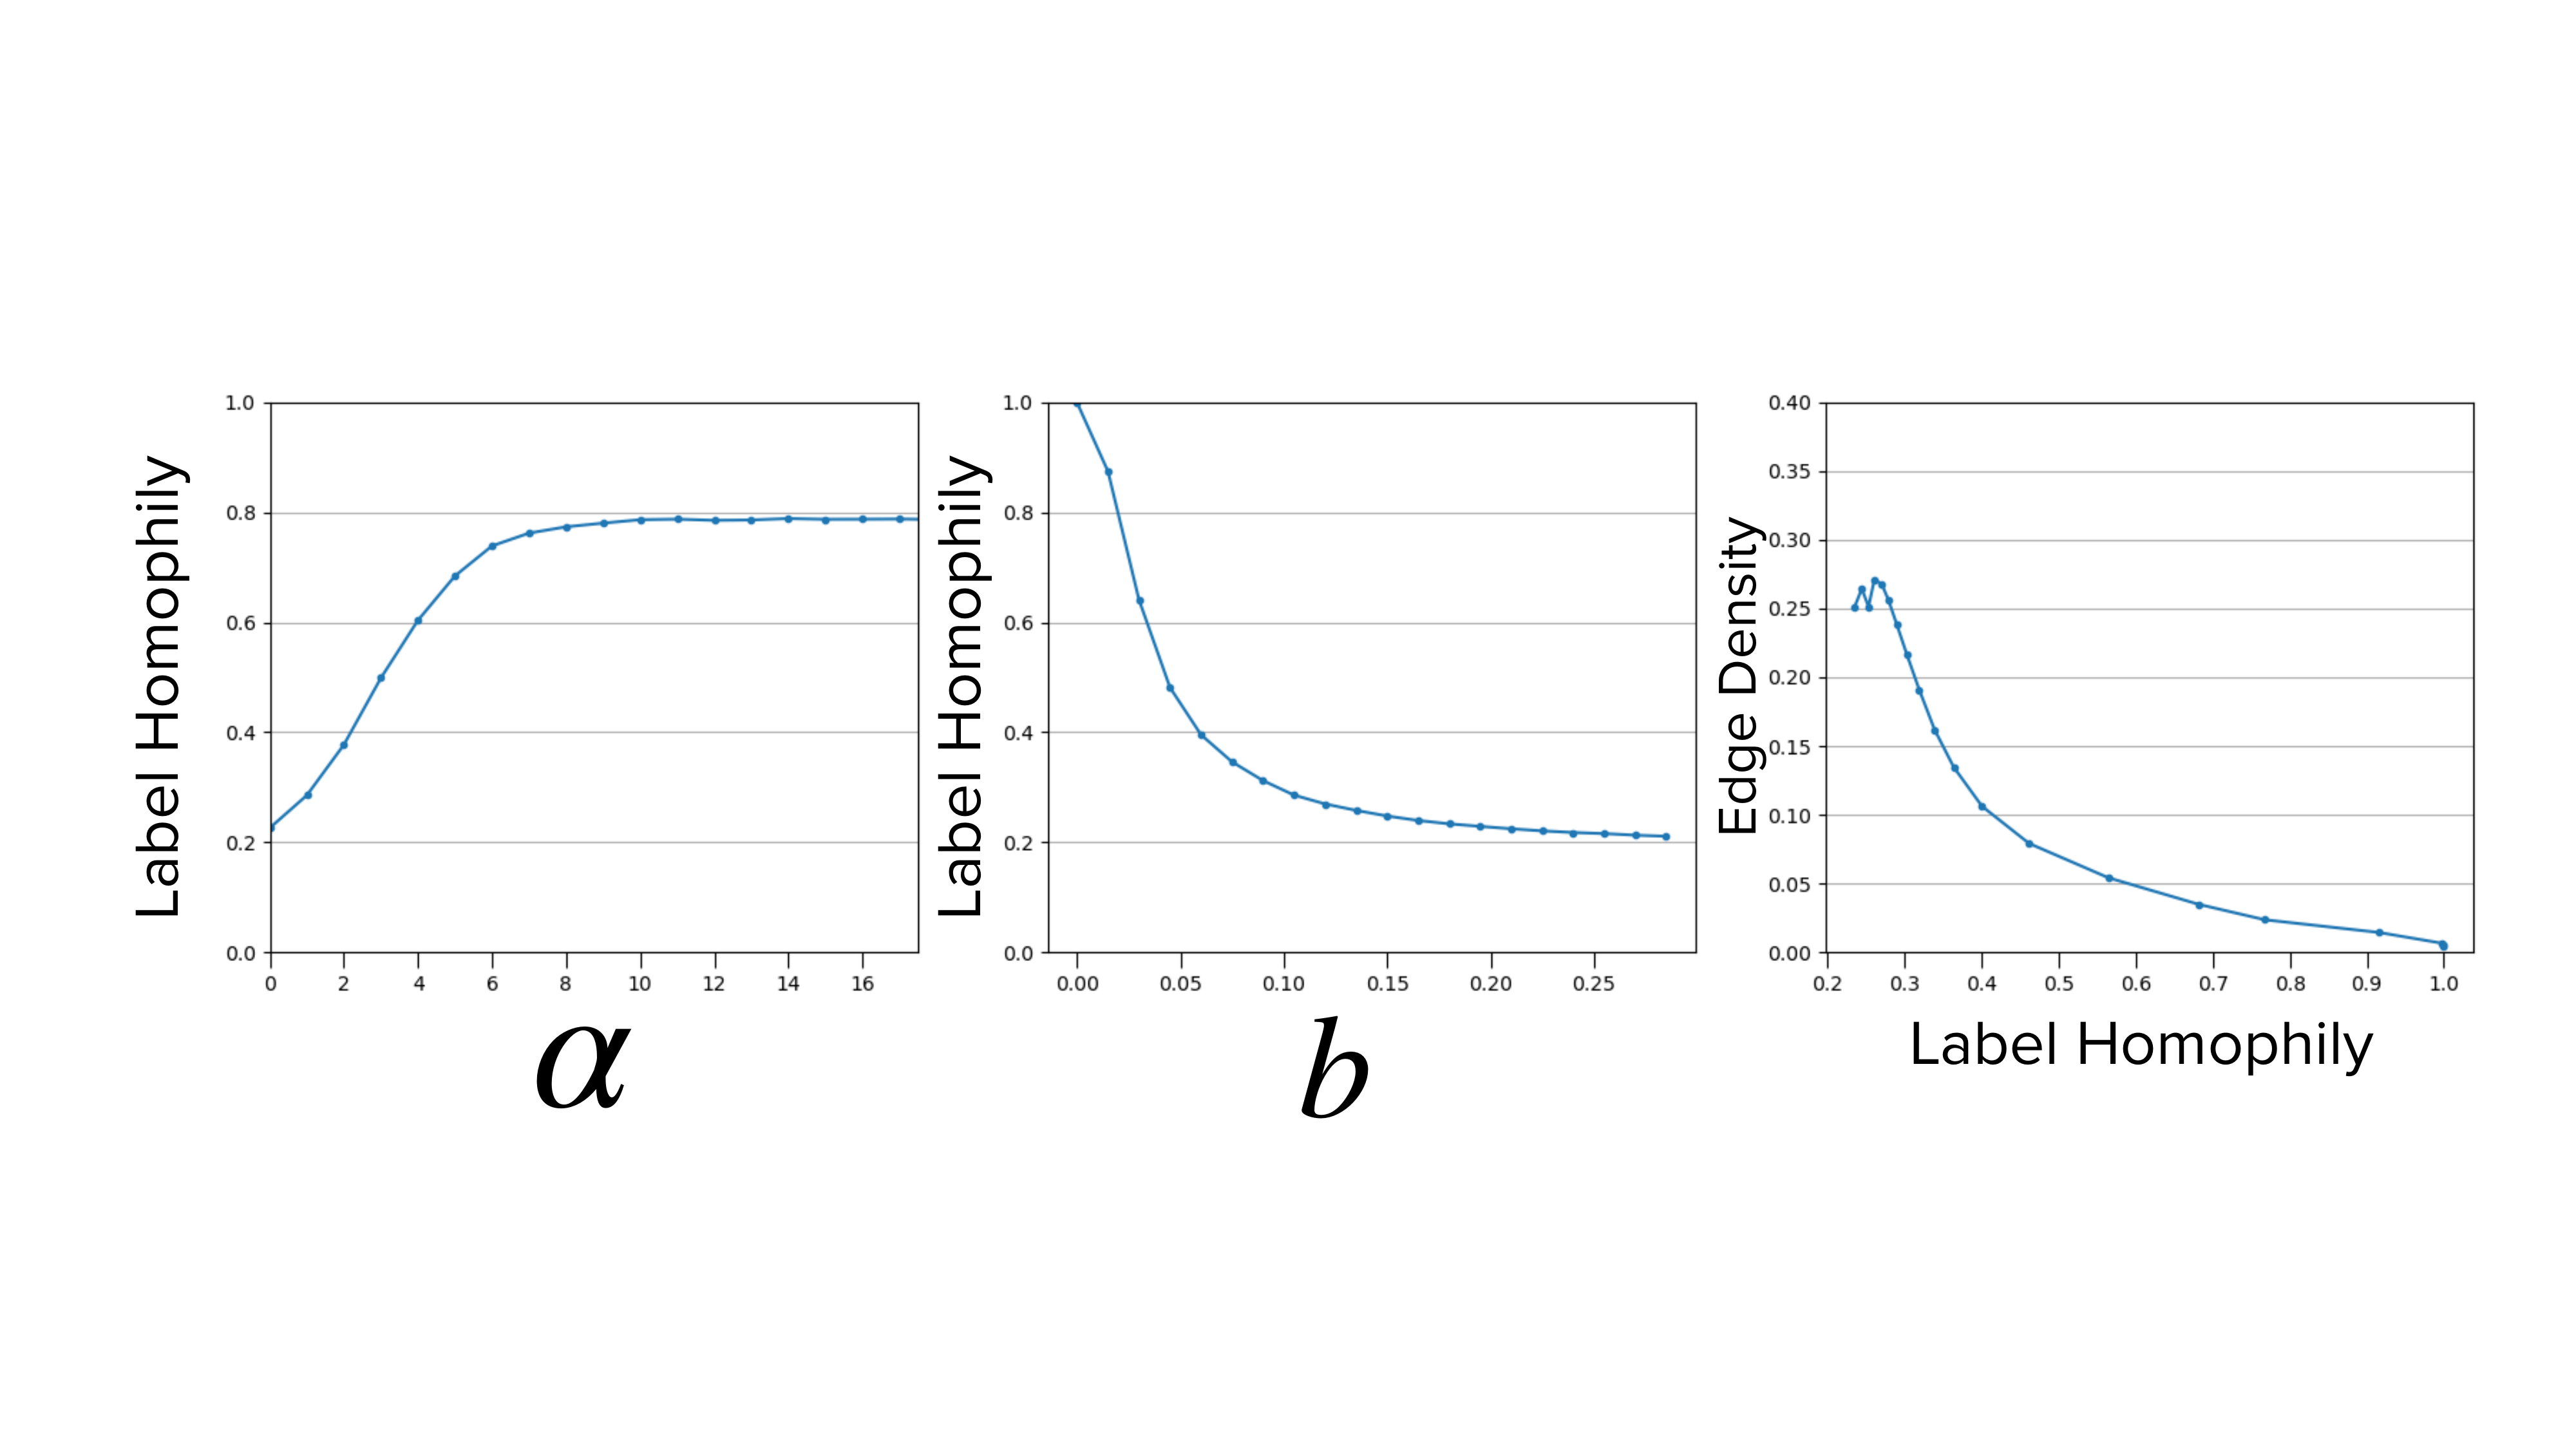}
    \caption{Visualization of the parameter study of the Graph Generator Model. The first two subplots demonstrate the relationships between the value of $\alpha$ and $b$ and the label homophily of the generated synthetic datasets. The last subplot shows the edge density and the label homophily of the generated synthetic graphs. This shows with the same multi-label data, we can generate synthetic graphs with varying label homophily.}
    \label{fig:my_label}
\end{figure}
As mentioned in Section \ref{Graph Genrator}, the choice of $\alpha$ and $b$ will directly determine the connection probability $p_{i,j}$ of each pair of nodes $i$ and $j$ and the homophily ratio of the generated synthetic graph. Here, we demonstrate how we choose the value of $\alpha$ and $b$ to generate synthetic graphs with varying homophily ratios. Note that the valid range of $\alpha$ and $b$ may differ when a different distance metric is used. 

Firstly, we randomly choose $500$ nodes from \textsc{Synthetic1} dataset and generate a series of small synthetic graphs with varying $\alpha$ and $b$ and observe the relationship between them. Since we have two hyperparameters' ranges to determine, we first fix the value of one and explore the range of the other and then vice versa. To recall, $b$ indicates the characteristic distance at which $p_{ij}={1\over 2}$, and our hamming distance should be in the range of $[0, 1]$, we first fix $b$ to $0.05$. We chose a small value of $b$ because the larger value of $b$ would dominate the influence of $\alpha$ and the relationship between the homophily ratio and the change of the value of $\alpha$ becomes unclear. The relationship between the homophily ratio of the generated synthetic graphs and the value of $\alpha$ is shown in Figure \ref{fig:my_label}(a). As shown in the subplot, the label homophily  increases monotonically as the value of $\alpha$ increases in the range of $[0, 10]$. As $\alpha$ is interpreted as the homophily parameter in \citep{boguna2004models}, only positive values make sense.

Similarly, we then fix $\alpha$ to its middle value in the valid range, i.e. $5$, and explore the valid range of $b$ and visualize the relationship of the graph level homophily ratio and the value of $b$ in Figure \ref{fig:my_label}(b). As illustrated in the subfigure, the label homophily decreases as the b increases in the range of $(0, 0.25]$. As $b$ increases, the node pairs with bigger distance would also have $50$\% of the probability to be connected, the number of edges will increase, and the label homophily ratio will decrease. As $b$ decreases, the node pair with a smaller distance would only have $50$\% of the probability of being connected. The model becomes cautious about connecting a node pair. The number of edges decreases and only the node pairs, which are alike will be connected, thus, the label homophily ratio increases.

Then, we use combinations of $\alpha$ and $b$ to generate synthetic graphs with specific homophily ratios. We sample 20 $\alpha$s and $b$s uniformly from their valid ranges with the increments 0.5 and 0.0125. Since the graph label homophily has an inverse linear relationship with $\alpha$ and $b$, we arrange the sampled $b$ in reverse order and then form 20 value pairs (alpha, b). We generate $20$ synthetic graphs from the multi-label dataset corresponding to \textsc{Synthetic1} with these value pairs ($\alpha$, $b$) and plot the homophily ratio and the edge density of the generated graphs in Figure \ref{fig:my_label}(c). As shown in the subplot, using the same multi-label data, we are able to generate synthetic graphs with varying homophiles. And the edge density decreases when label homophily increases. As in higher label homophily graphs, the generator will only connect the nodes that are highly similar to each other. In contrast, when the label homophily is low, the graph generator will connect every possible node pair in the graph resulting in denser graphs.

\subsubsection{Statistics Of The Synthetic Datasets}
Here we summarize the characteristics of the generated synthetic graphs with varying label homophily and feature quality. The first row denotes the name of the synthetic graphs, where in the varying homophily experiments, the variants of datasets are named with their label homophily. The \textsc{Synthetic1} dataset is used in the varying feature quality experiment, where we remove the relevant features to create dataset variants with varying feature quality levels. Note that for all the datasets the label distribution stays the same as they are just different graphs generated from the same multi-label dataset. The statistics on label distribution for these datasets are given in Table \ref{Tab: statis_syn} and Table \ref{Tab: labeldist_syn}.

\label{statis_syn}

\begin{table}[!h]

\caption{The number of edges and clustering coefficient of the synthetic datasets with varying label homophily and \textsc{Synthetic1}. The row of '|E|' denotes the number of edges and the 'clustering coefficient' denotes the clustering coefficient of these datasets}
\centering
\begin{tabular}{c|c|c|c|c|c|c}
\hline
Dataset & 0.2     & 0.4     & 0.6                         & 0.8    & 1.0   &\textsc{Synthetic1}\\ \hline
|E|             & 2.37M & 598k & \multicolumn{1}{l|}{298k} & 79.5k & 47.6k &1.00M\\ \hline
Clustering Coefficient     & 0.53    & 0.37    & 0.39                        & 0.49   & 0.93  &0.57\\ \hline

\end{tabular}
\label{Tab: statis_syn}
\end{table}

\begin{table}[!h]

\caption{The label distribution of the synthetic dataset used in this work. The column notations are same as in Table \ref{tab:dataset}. }
\centering
\begin{tabular}{c|c|c|c|c|c|c|c}
\hline
&$|L|$ &$|L_{med}|$& $|L_{mean}|$  & $|L_{max}|$& $25$\% & $50$\% & $75$\%\\ \hline
label distribution &20&3&3.23&12&1&3&5 \\ \hline

\end{tabular}
\label{Tab: labeldist_syn}
\end{table}

\begin{figure}
     \centering
     \begin{subfigure}[b]{0.3\textwidth}
        \centering
        \includegraphics[width=1.0\linewidth]{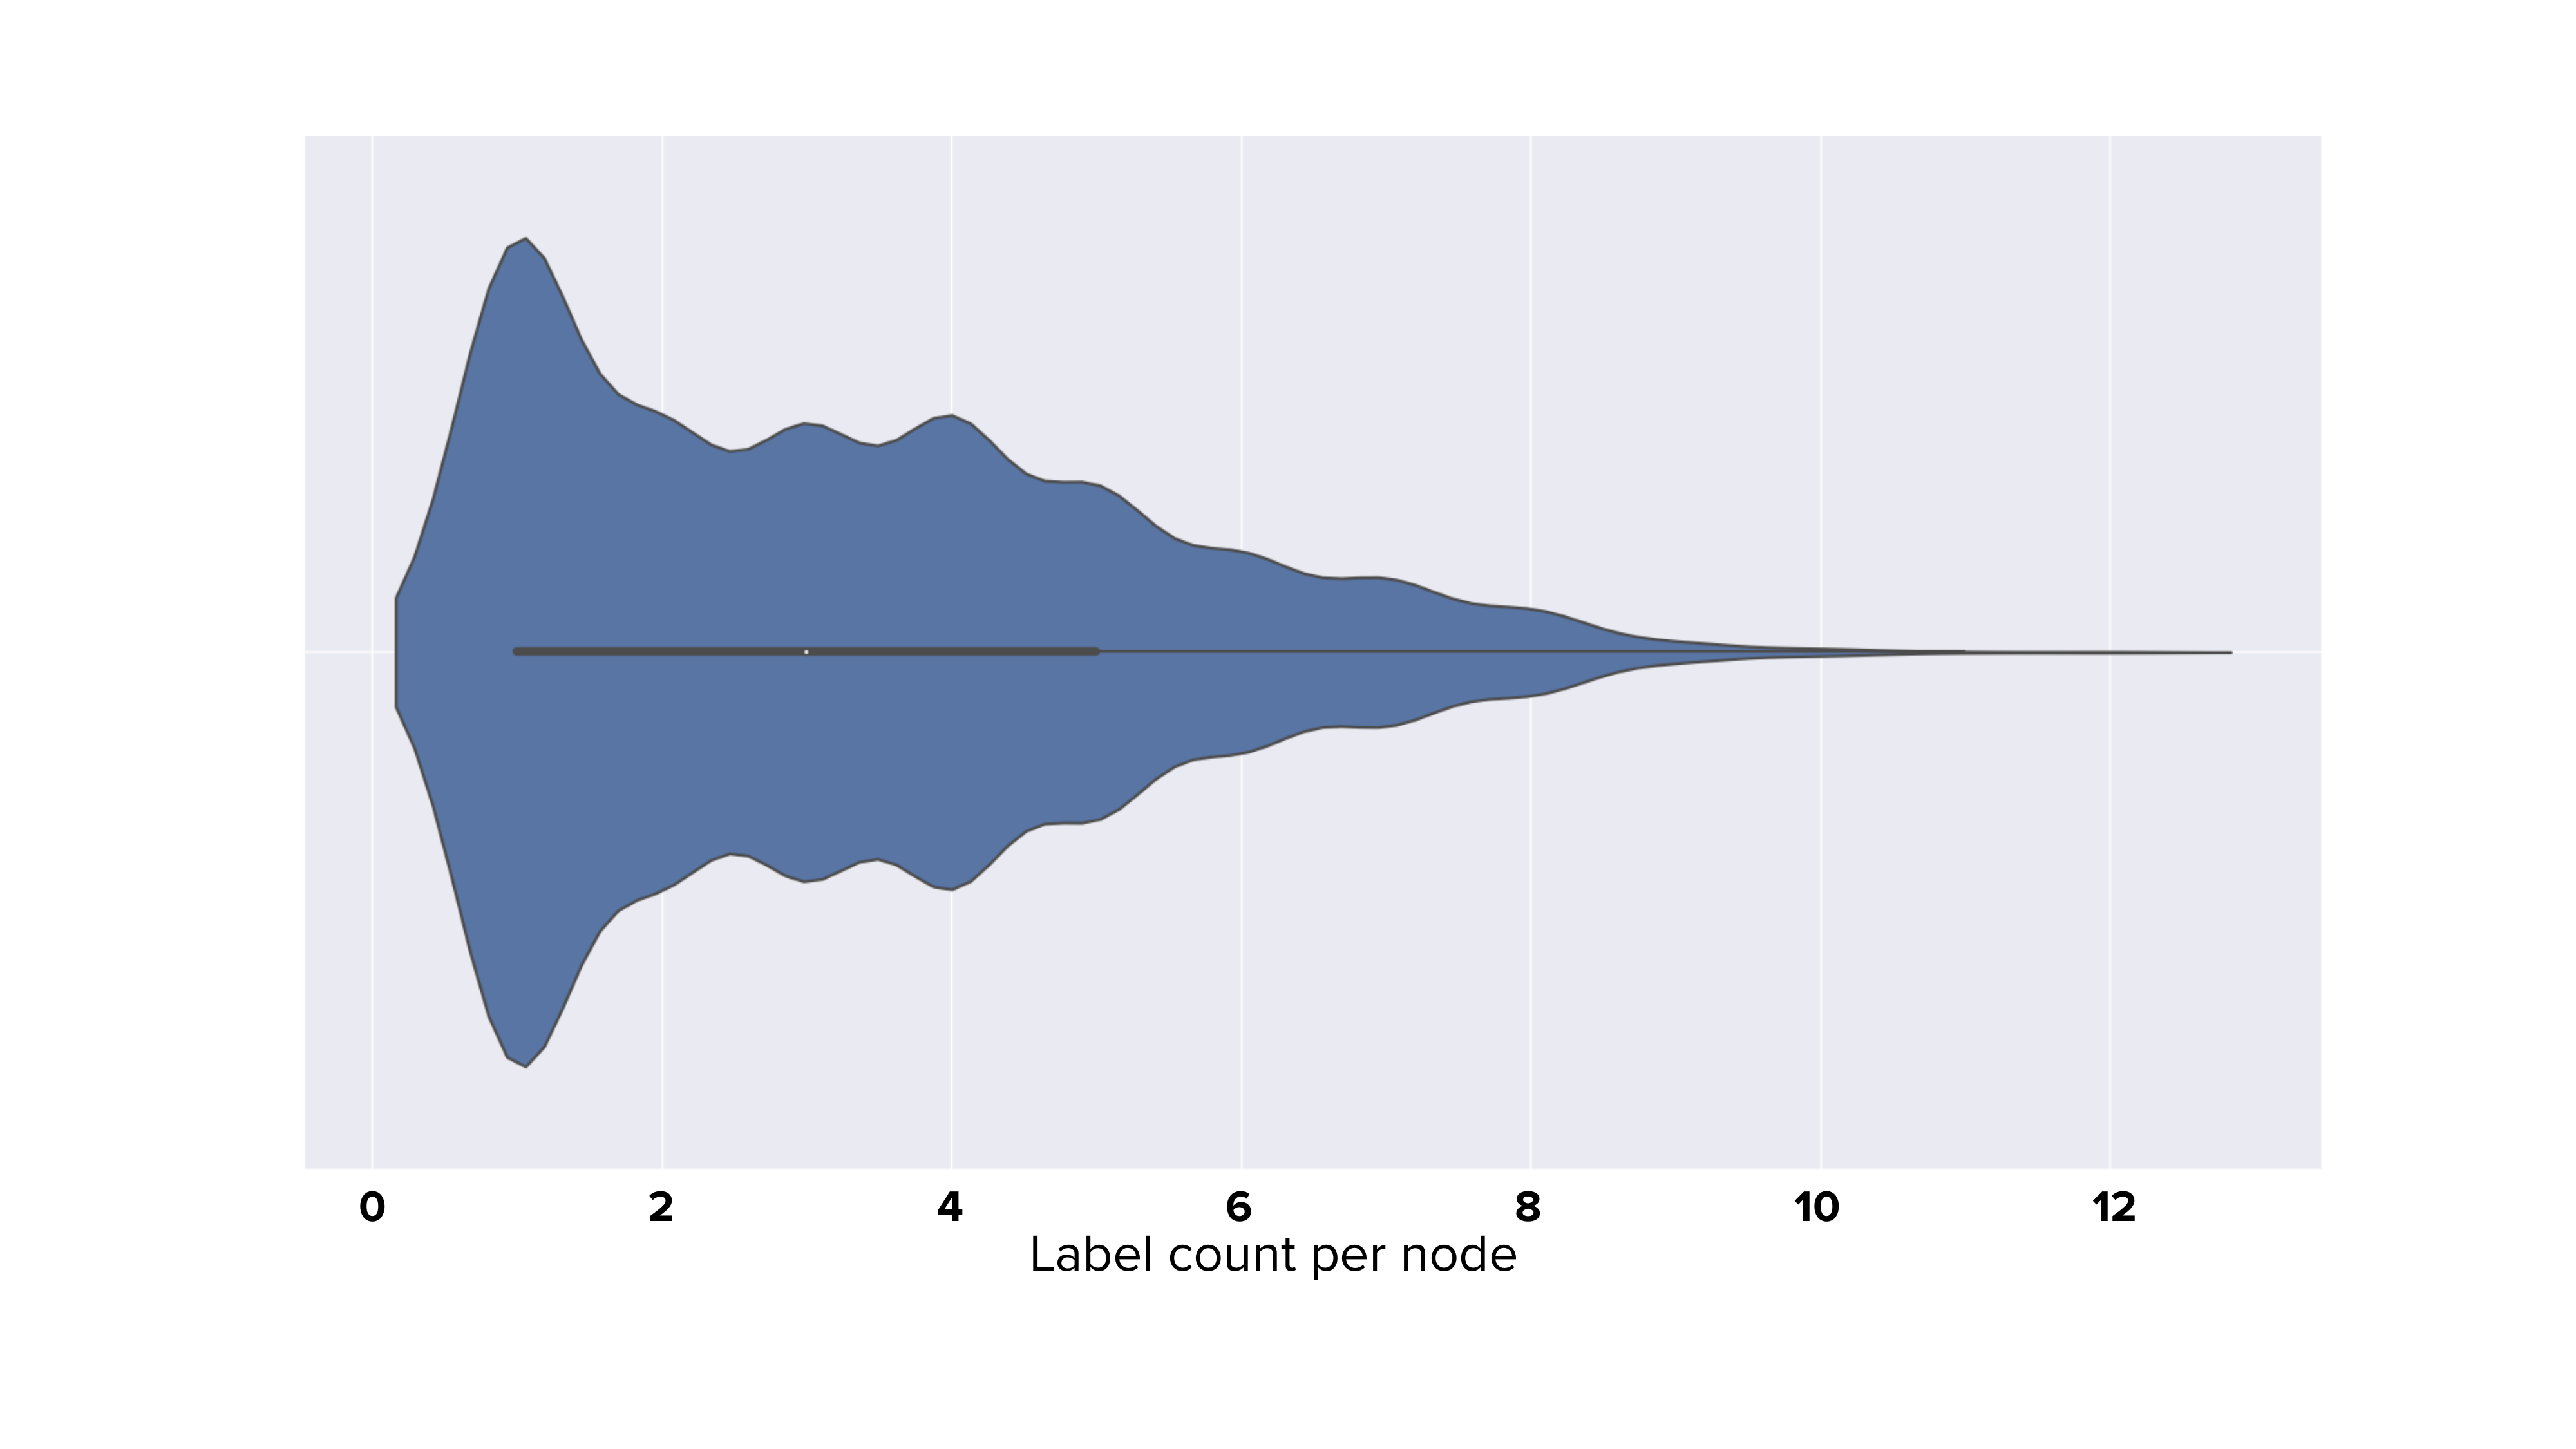}
        \caption{Label distribution in the synthetic dataset is more balanced. A relatively high multi-label character is exhibited with $50\%$ nodes having more than 3 labels.}
        \label{fig:labeldistsynthetic}
    \end{subfigure}
    \hfill
     \begin{subfigure}[b]{0.3\textwidth}
         \centering
         \includegraphics[width=\textwidth]{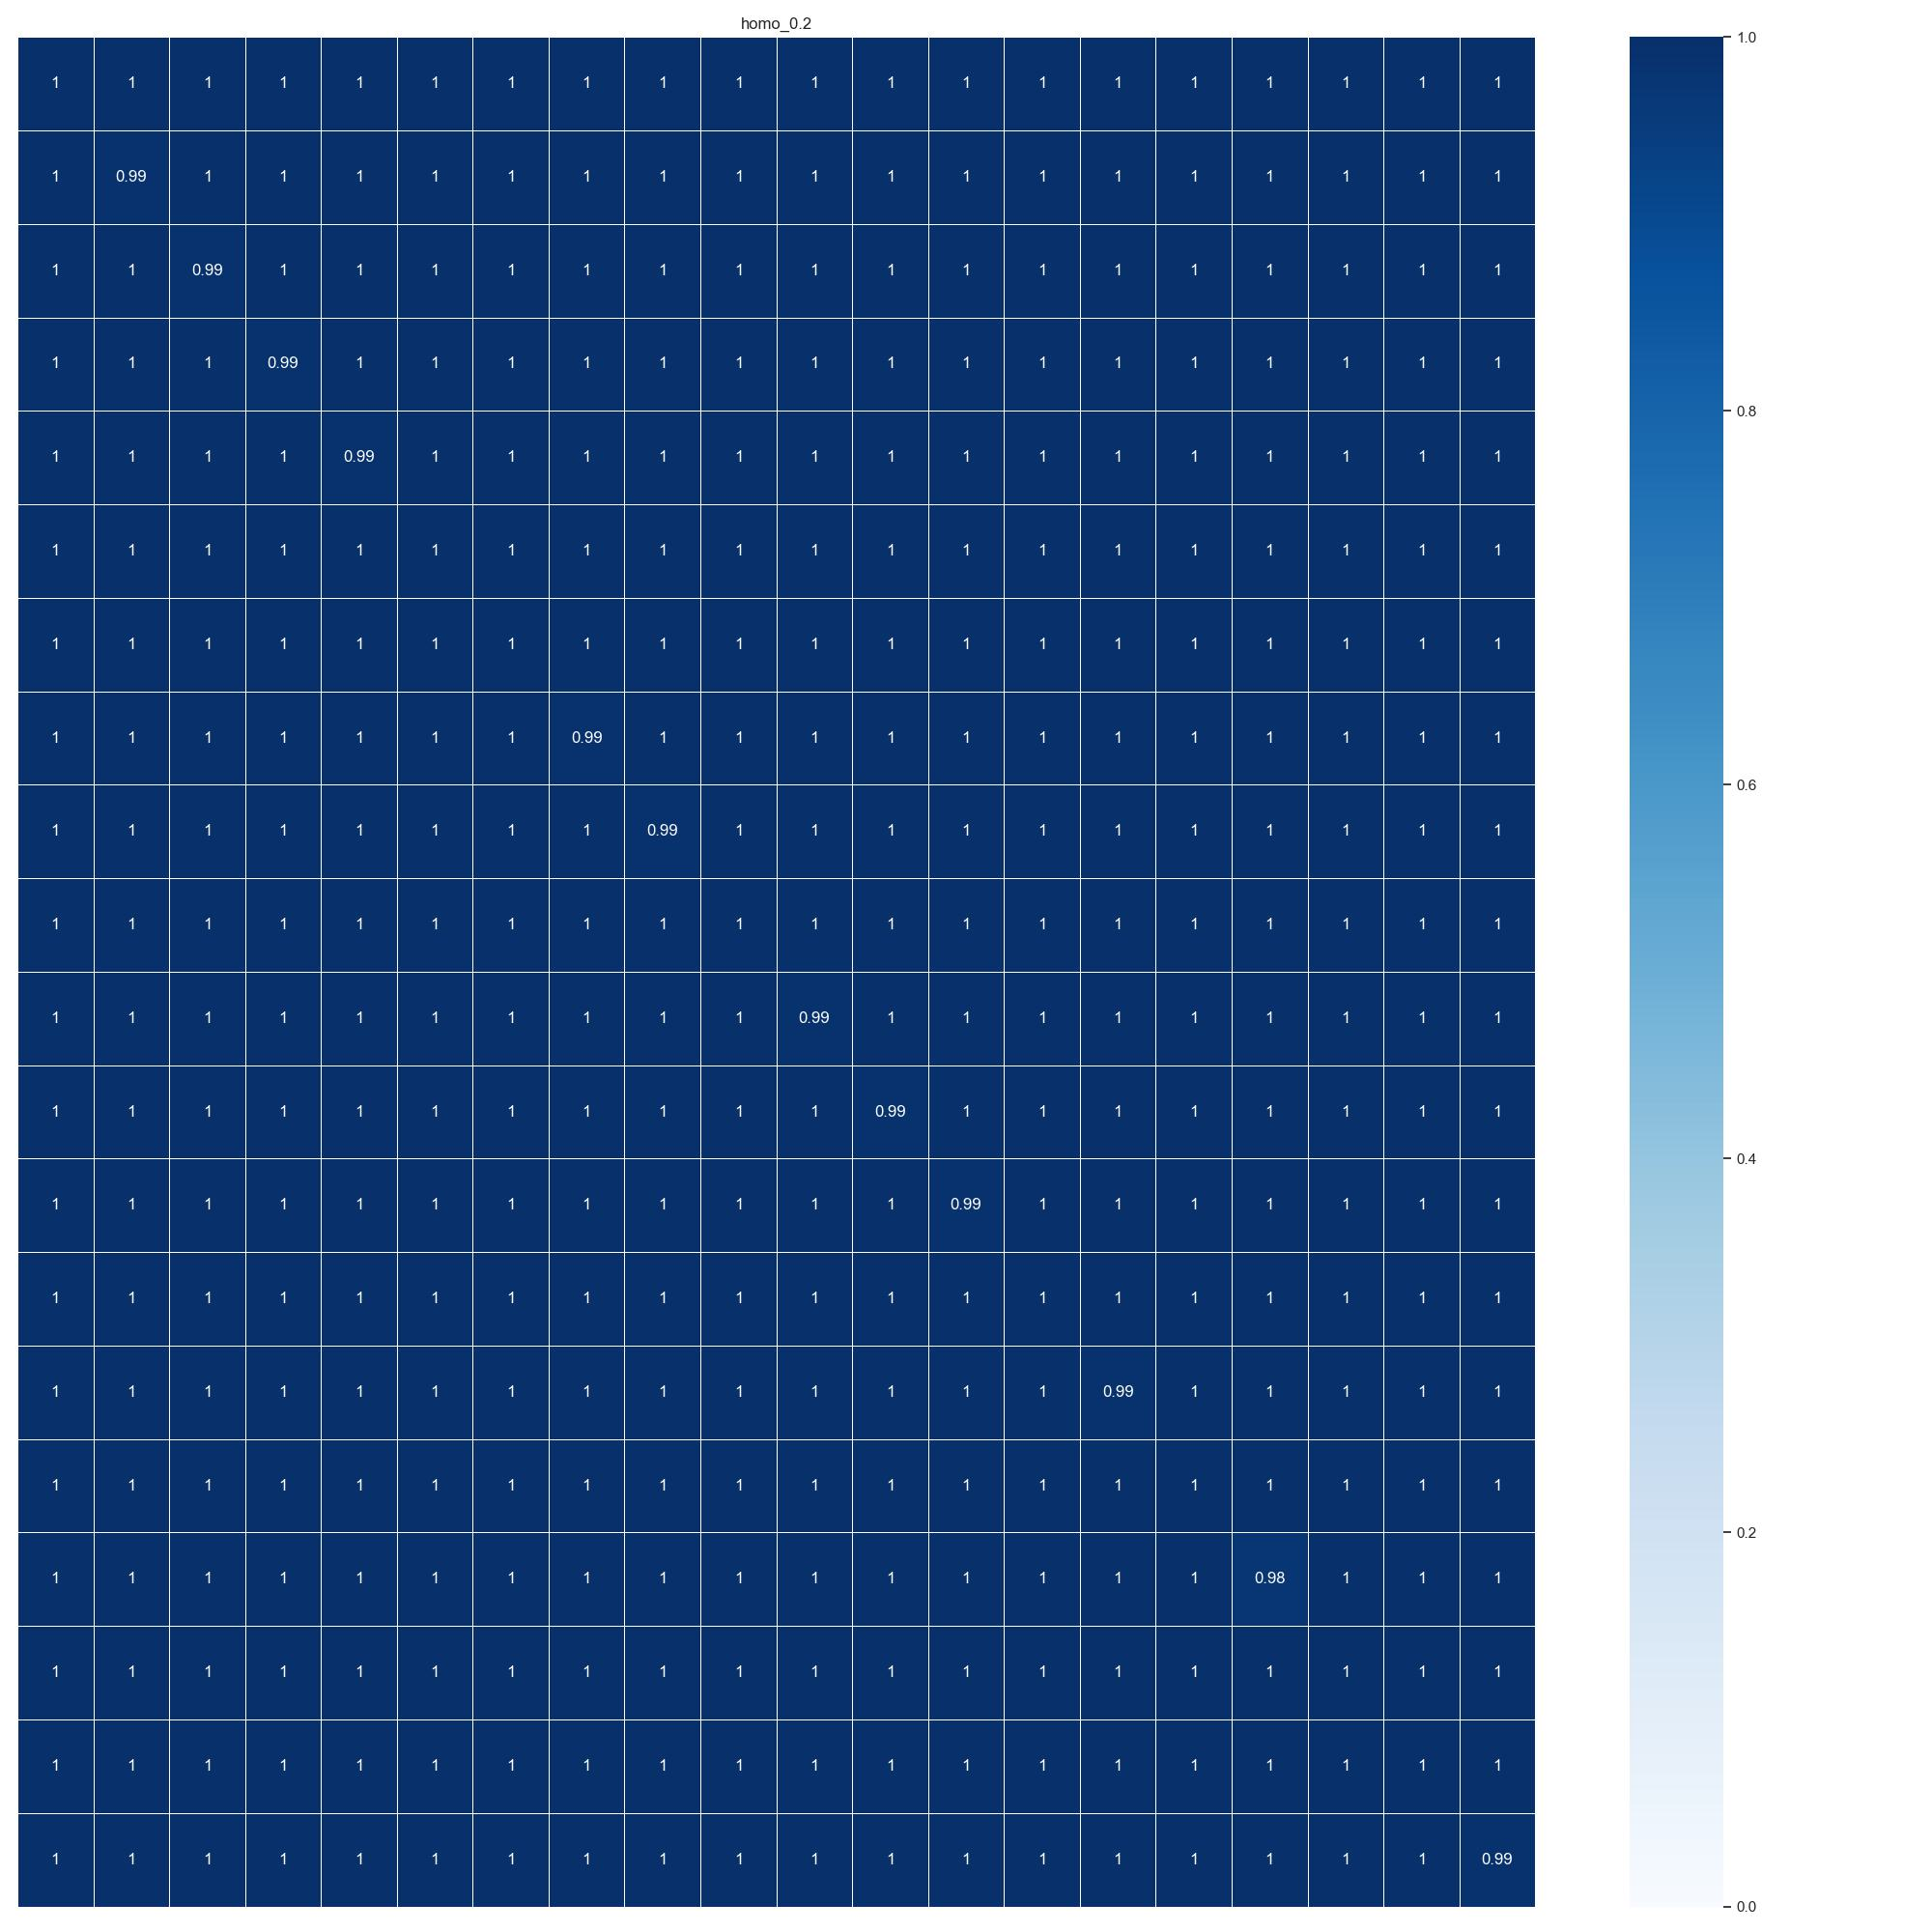}
         \caption{Cross-class Neighborhood Similarity in graph label homophily=0.2}
         \label{fig:ccns_0.2}
     \end{subfigure}
     \hfill
     \begin{subfigure}[b]{0.3\textwidth}
         \centering
         \includegraphics[width=\textwidth]{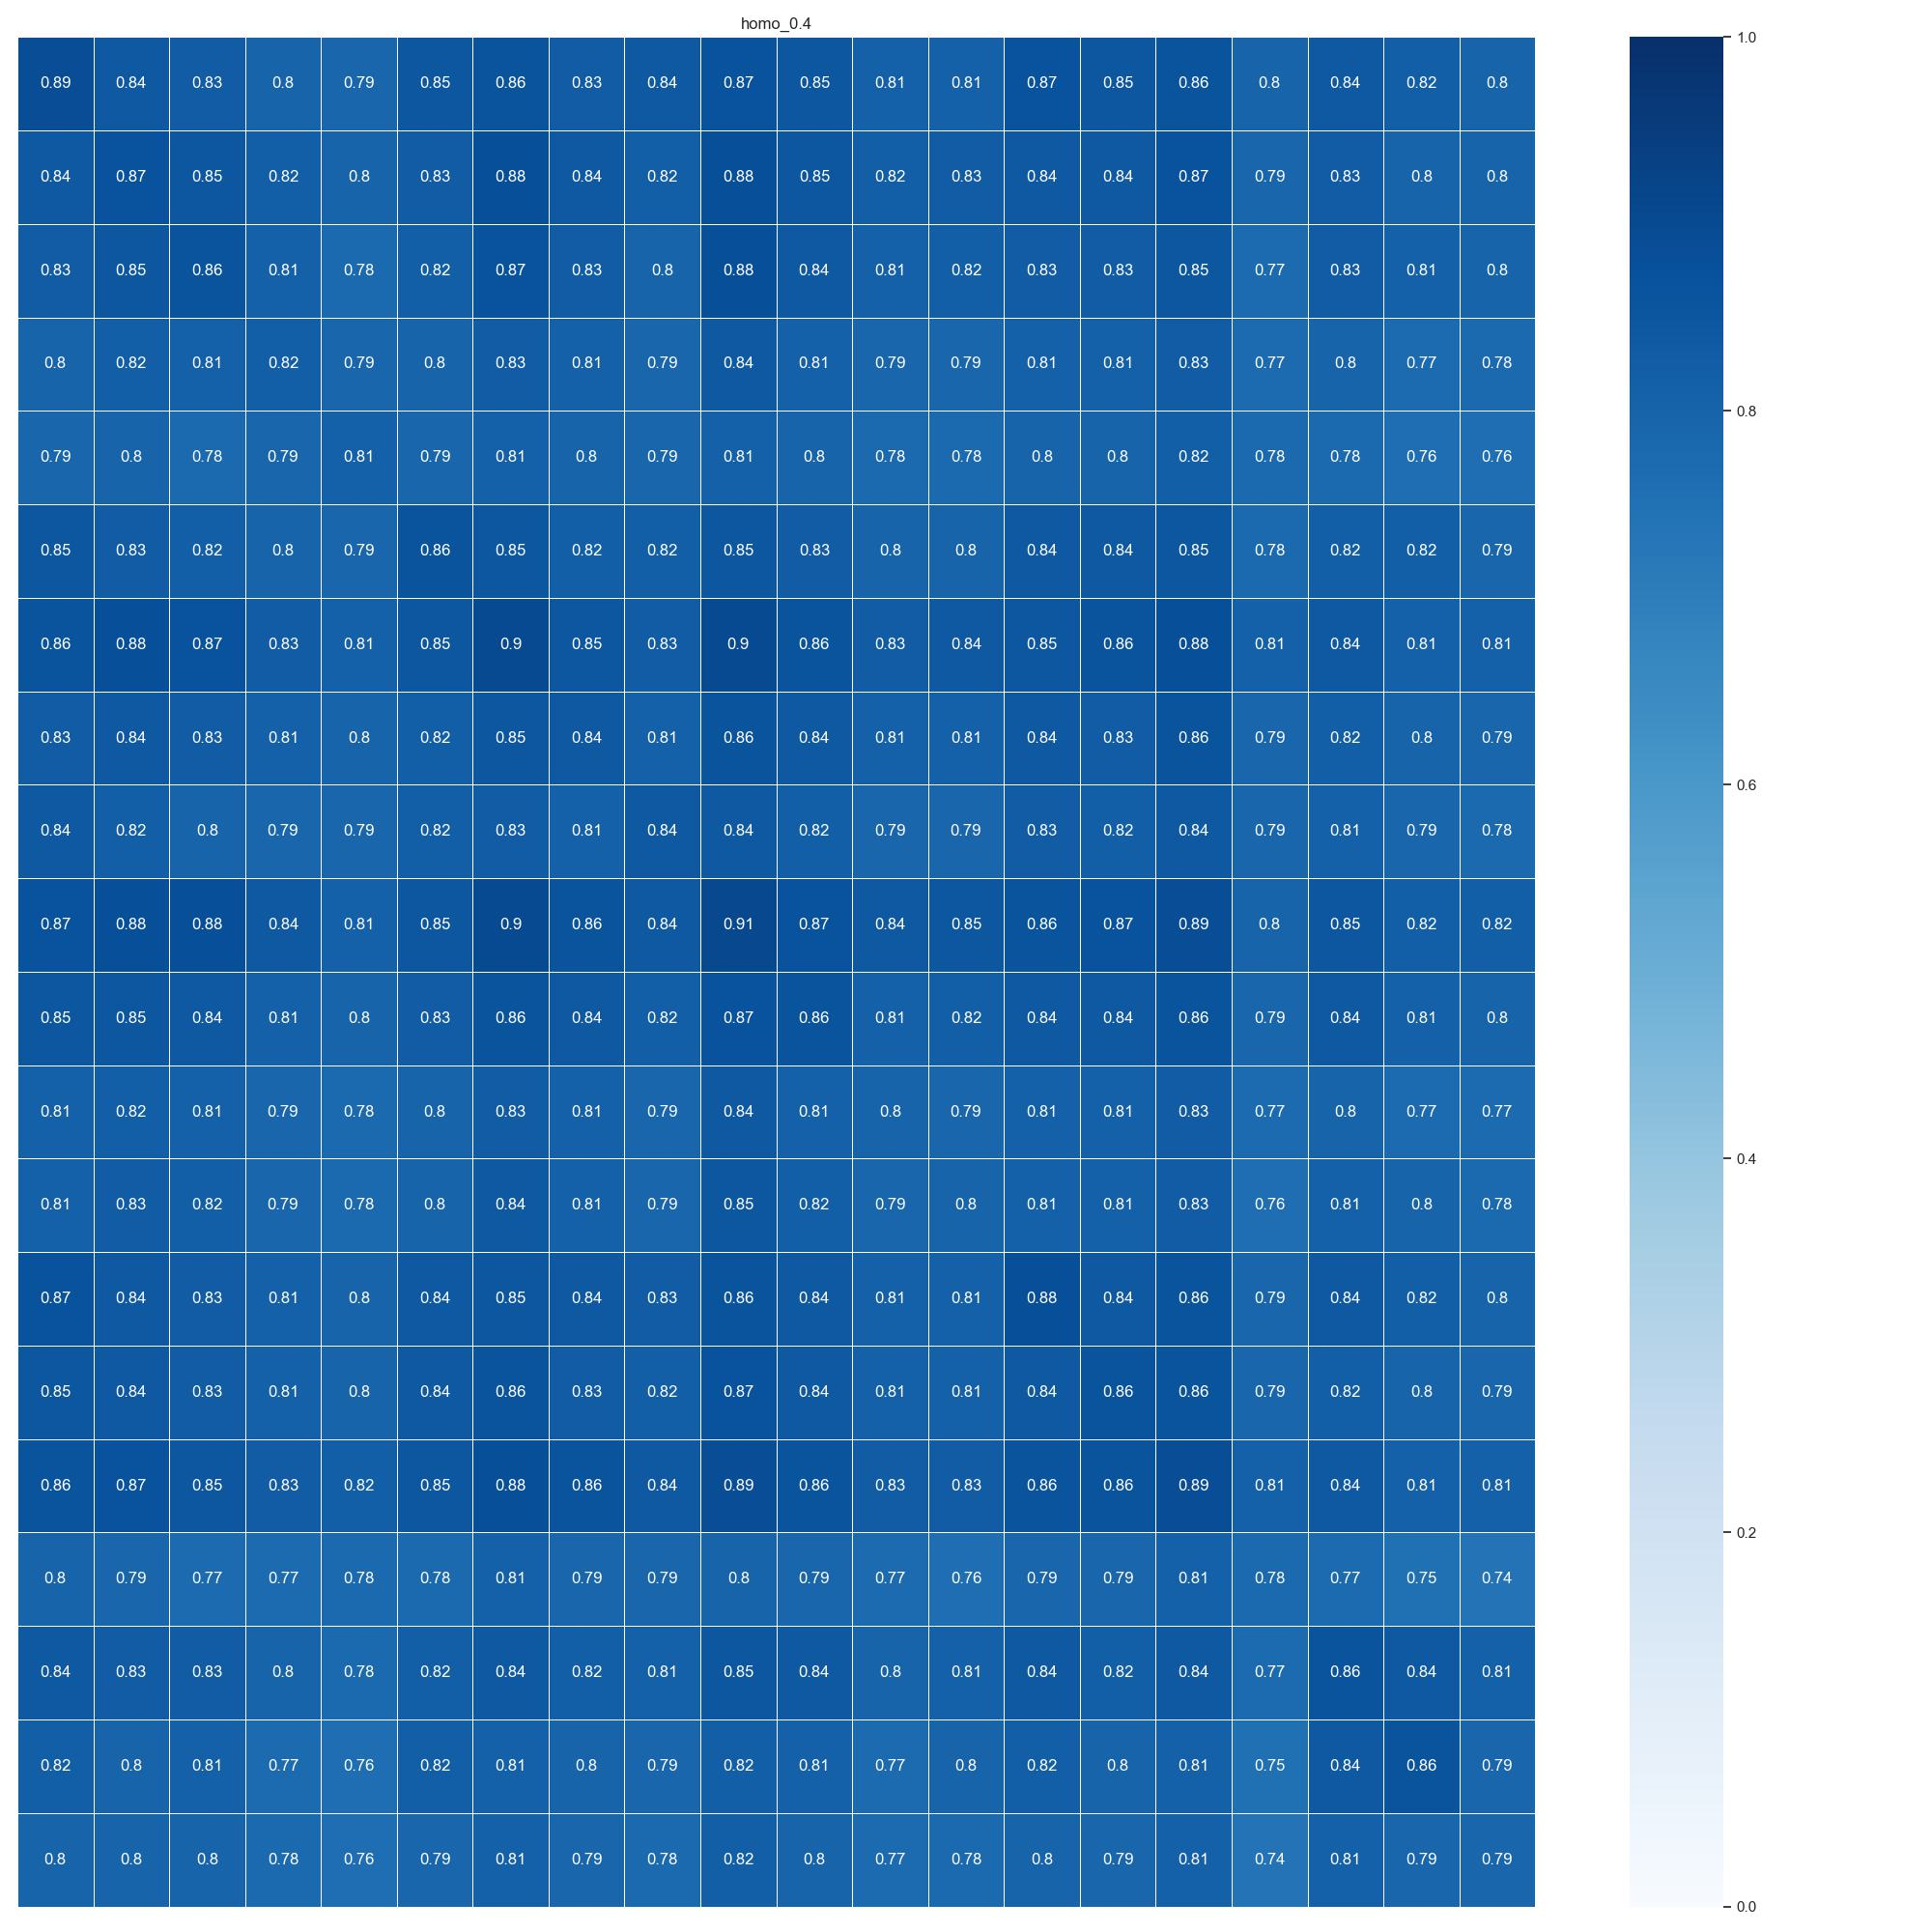}
         \caption{Cross-class Neighborhood Similarity in graph label homophily=0.4}
         \label{fig:ccns_0.4}
     \end{subfigure}
     \medskip
     \begin{subfigure}[b]{0.3\textwidth}
         \centering
         \includegraphics[width=\textwidth]{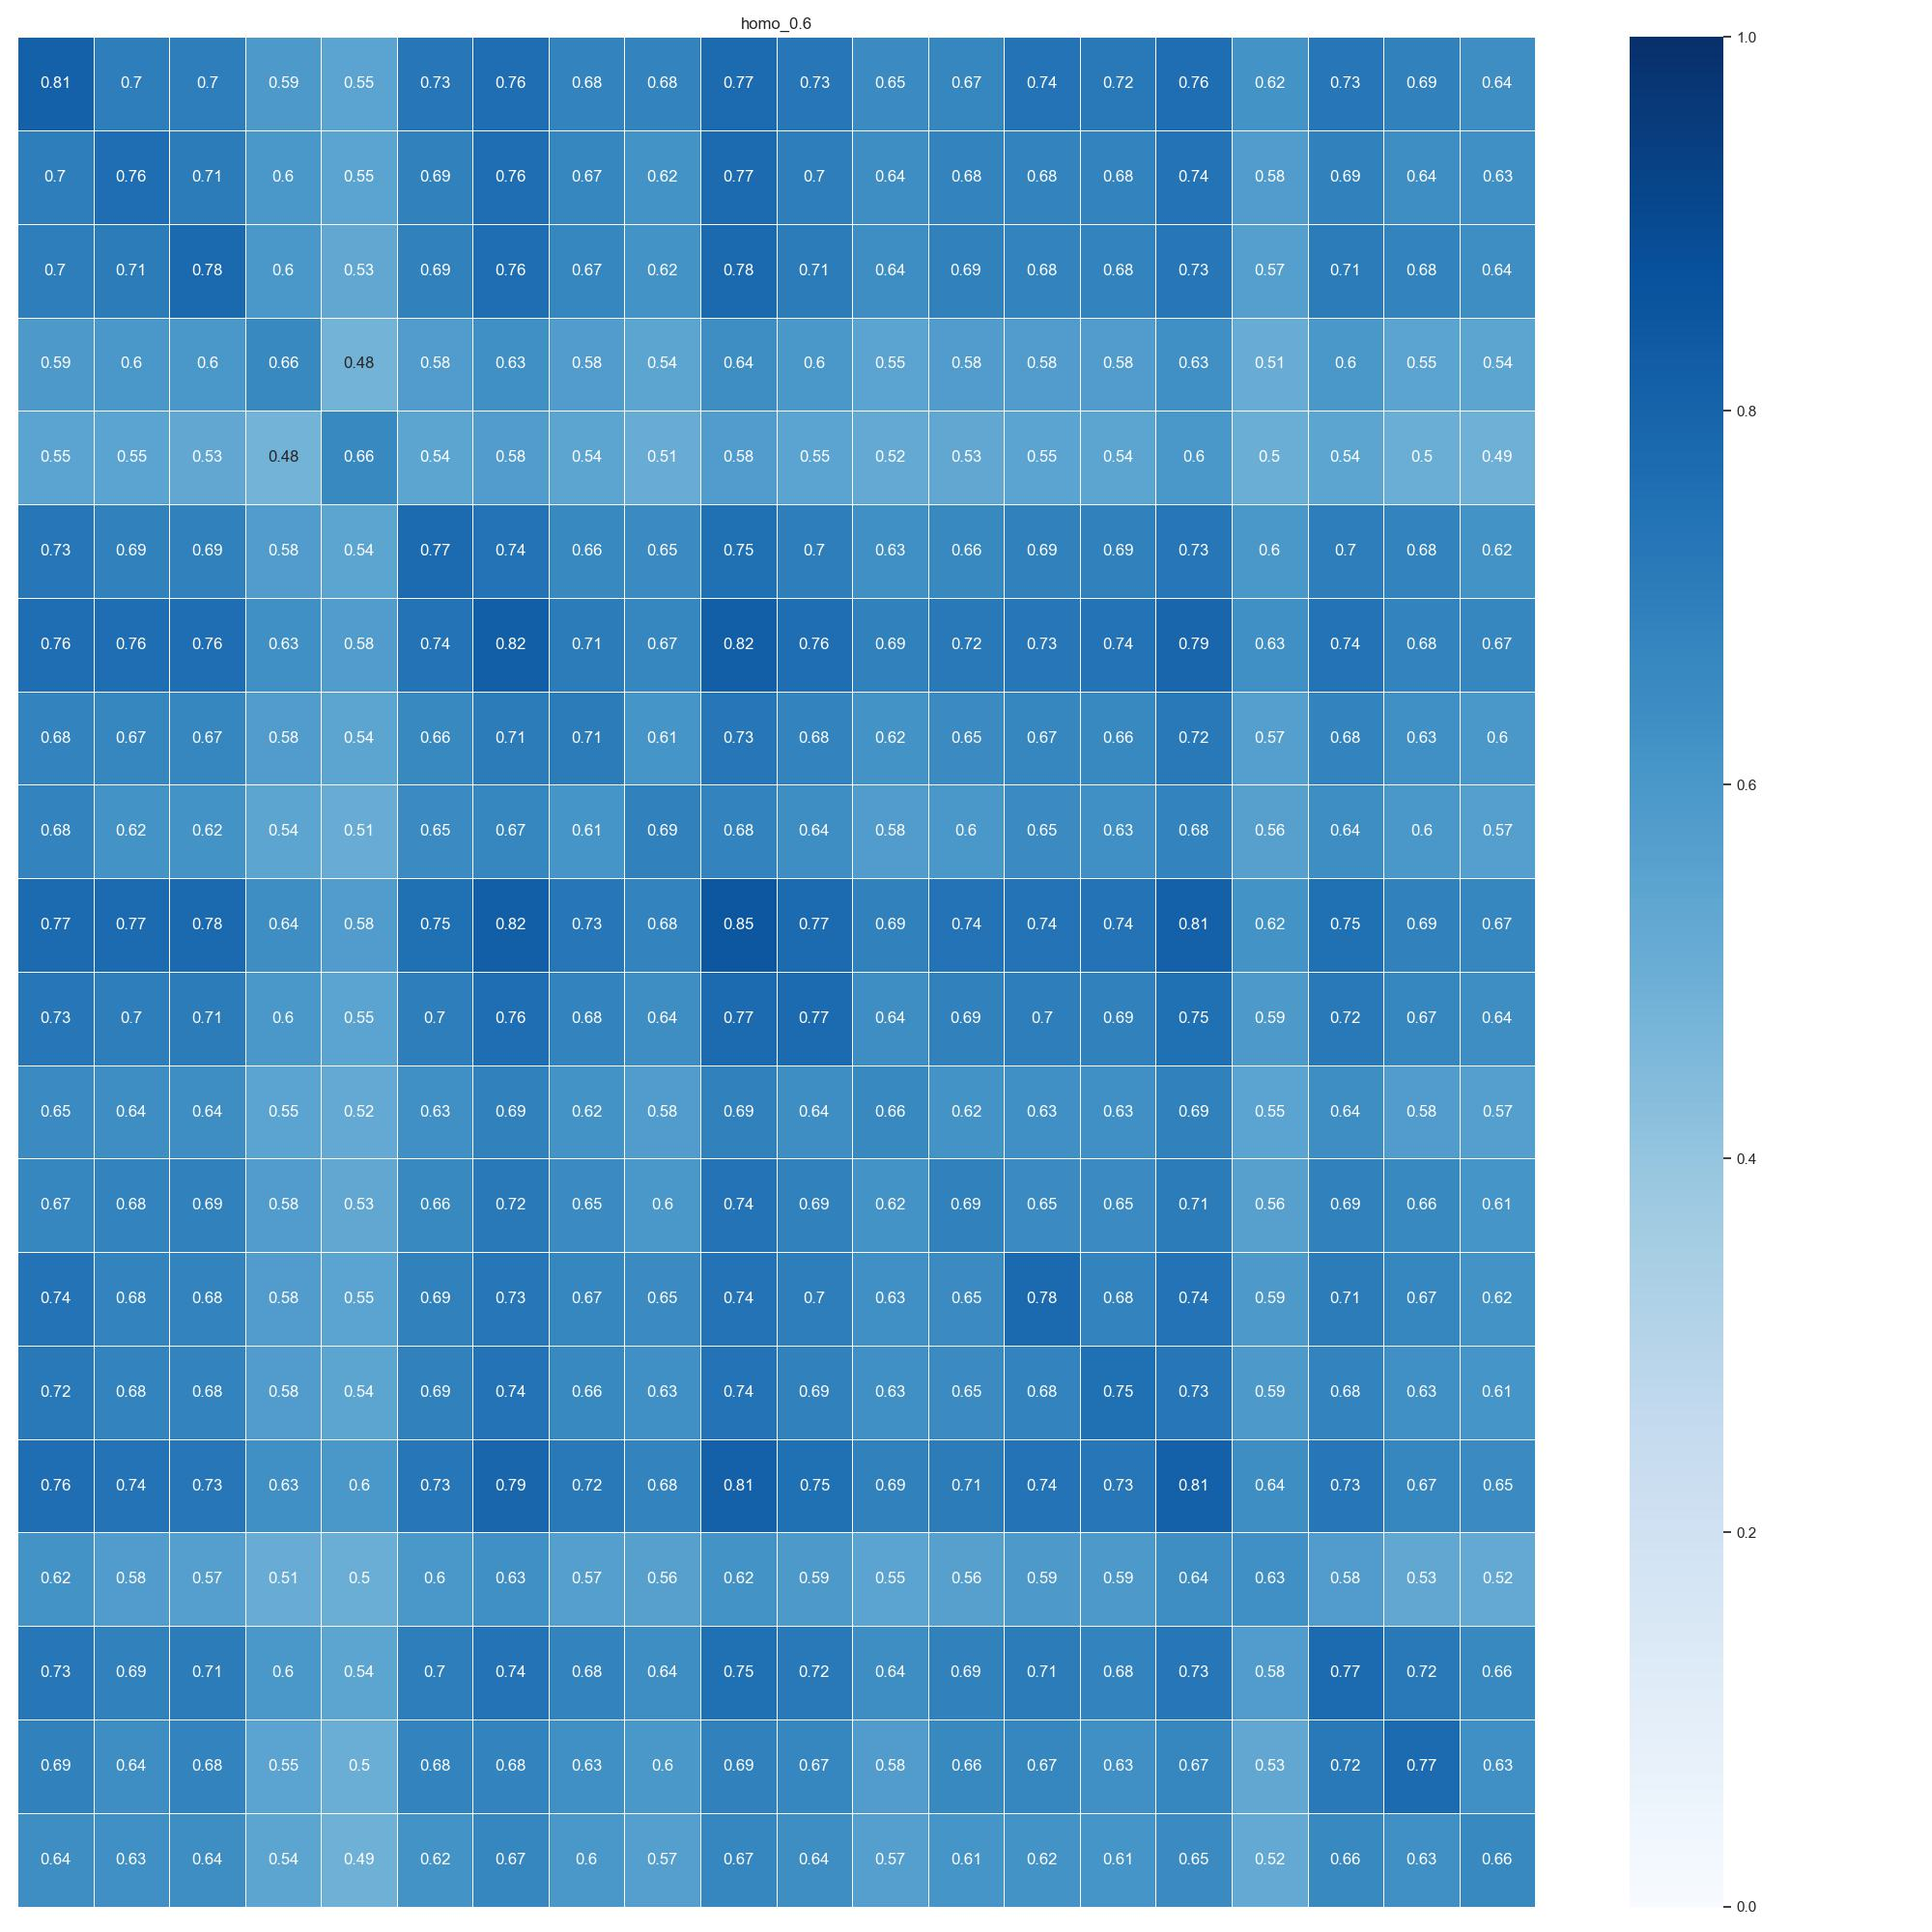}
         \caption{Cross-class Neighborhood Similarity in graph label homophily=0.6}
         \label{fig:ccns_0.6}
     \end{subfigure}
     \hfill
     \begin{subfigure}[b]{0.3\textwidth}
         \centering
         \includegraphics[width=\textwidth]{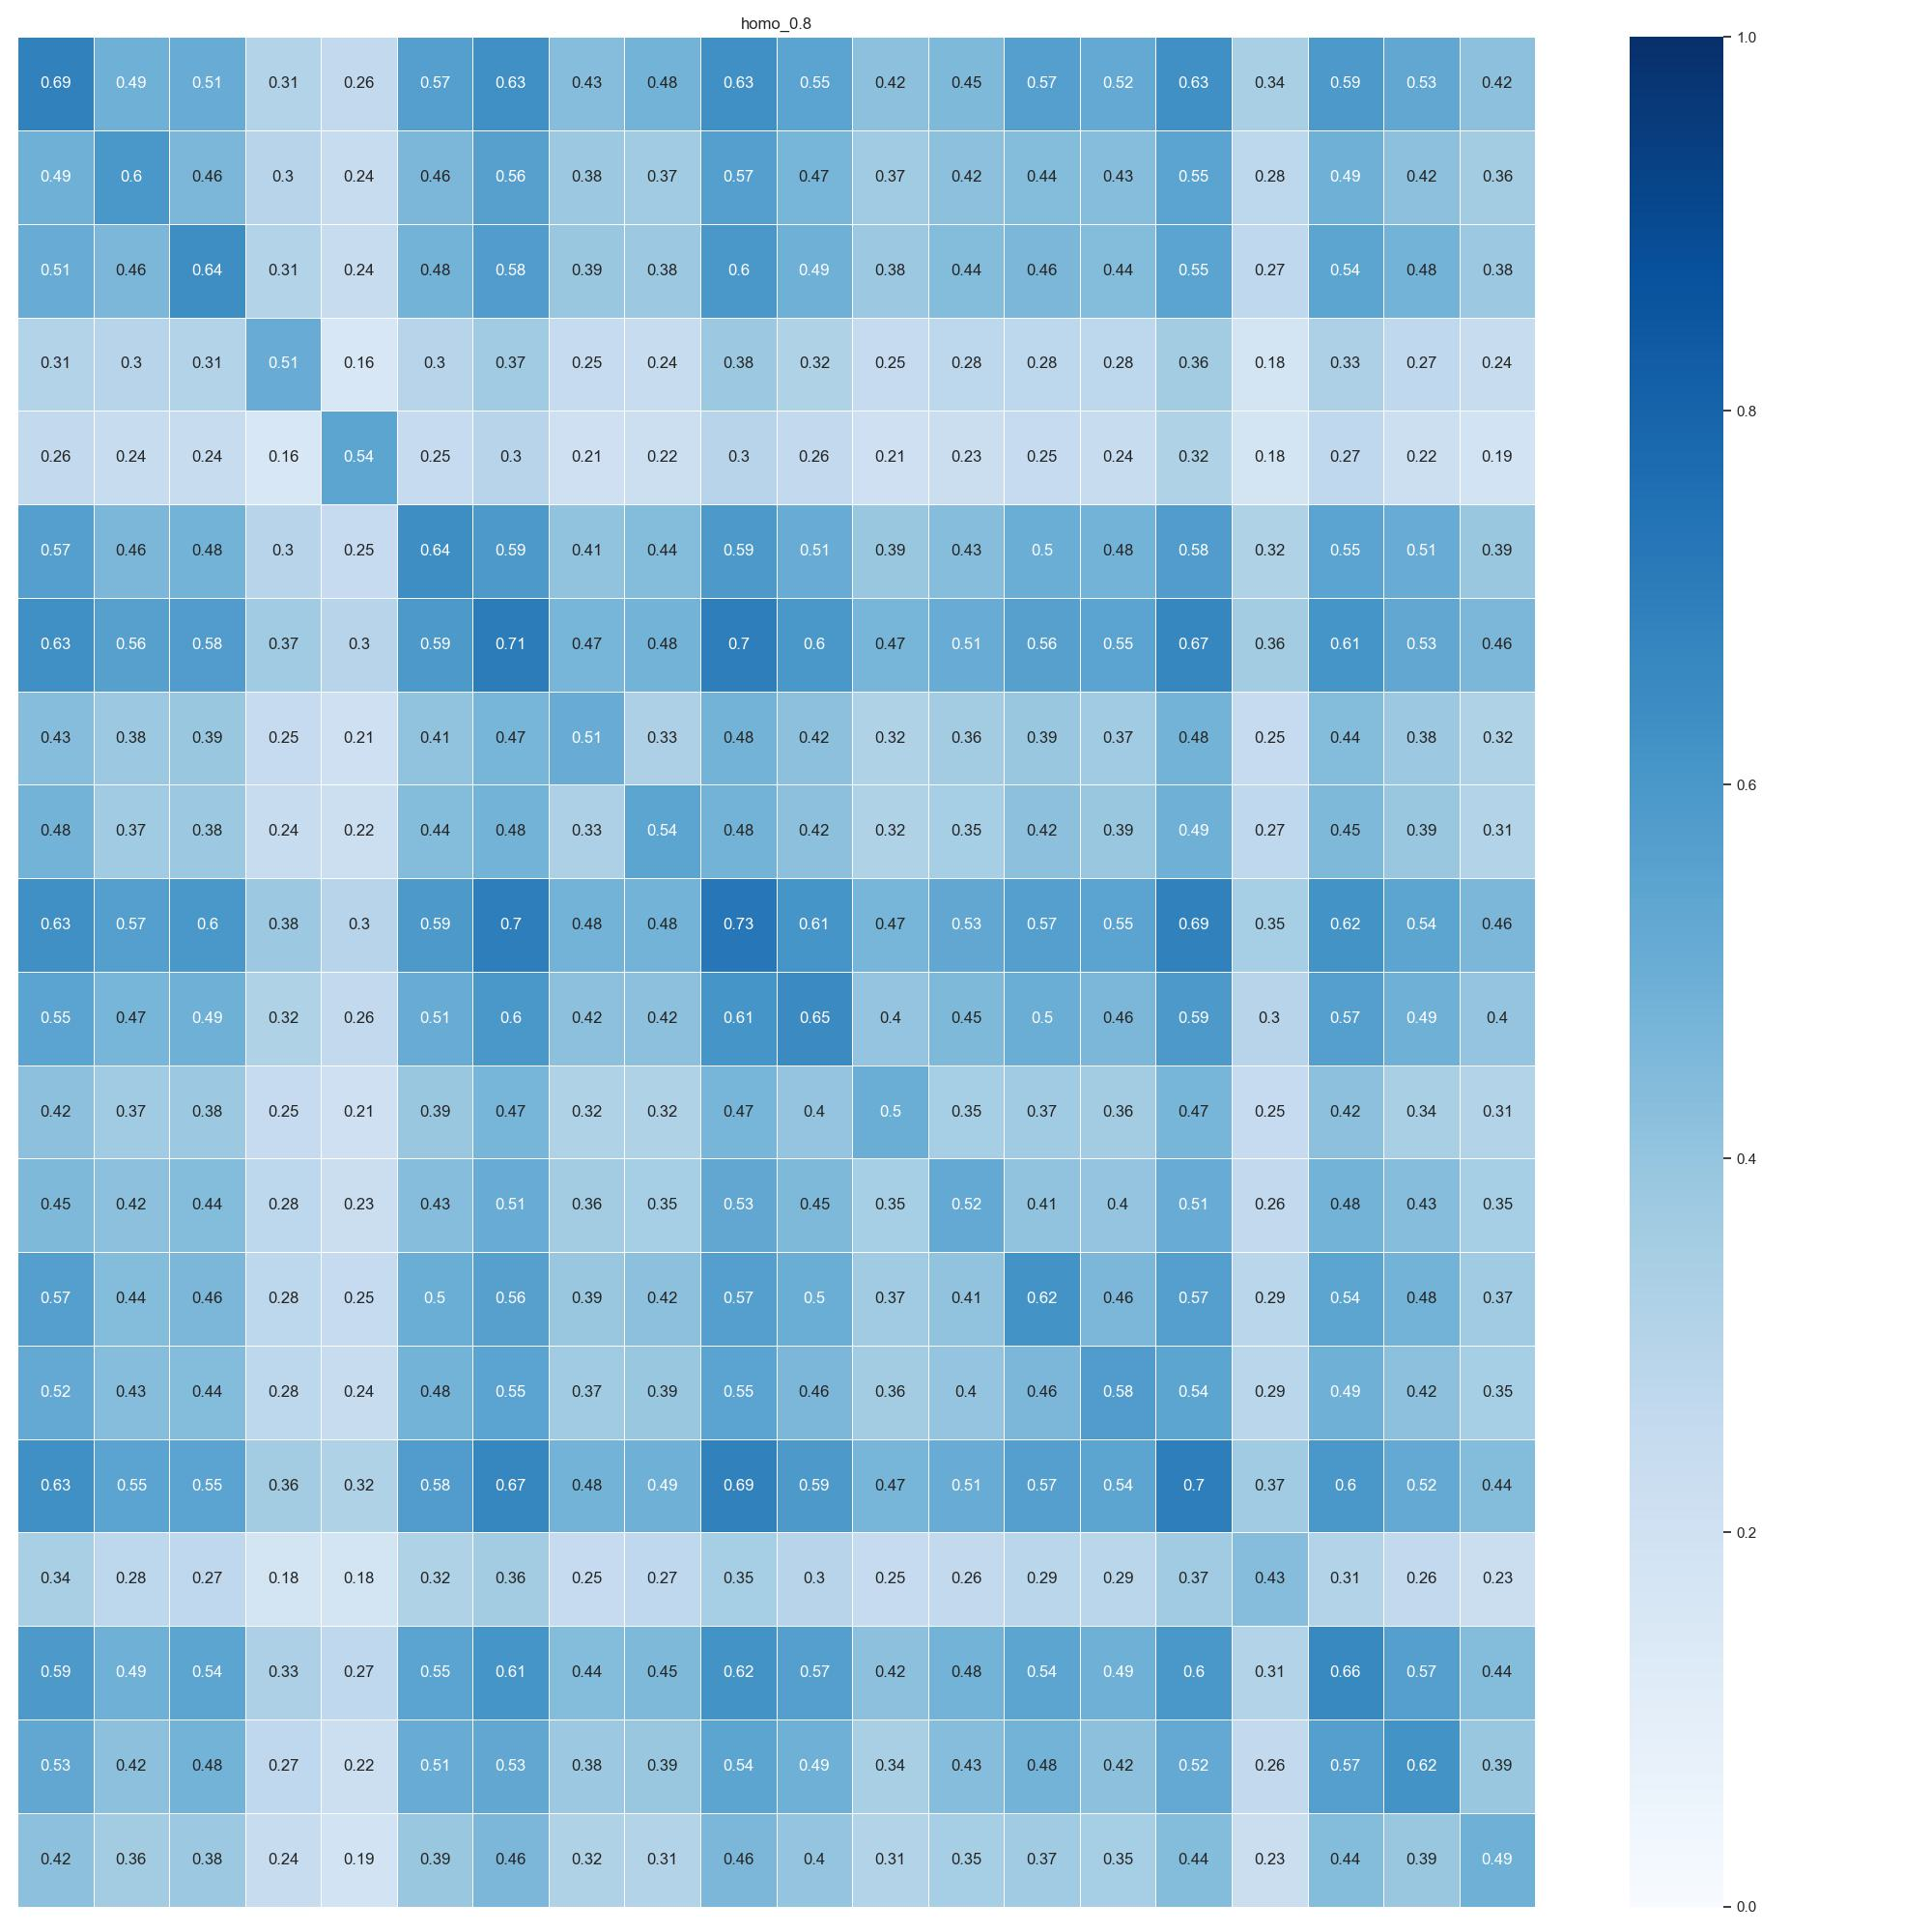}
         \caption{Cross-class Neighborhood Similarity in graph label homophily=0.8}
         \label{fig:ccns_0.8}
     \end{subfigure}
     \hfill
     \begin{subfigure}[b]{0.3\textwidth}
         \centering
         \includegraphics[width=\textwidth]{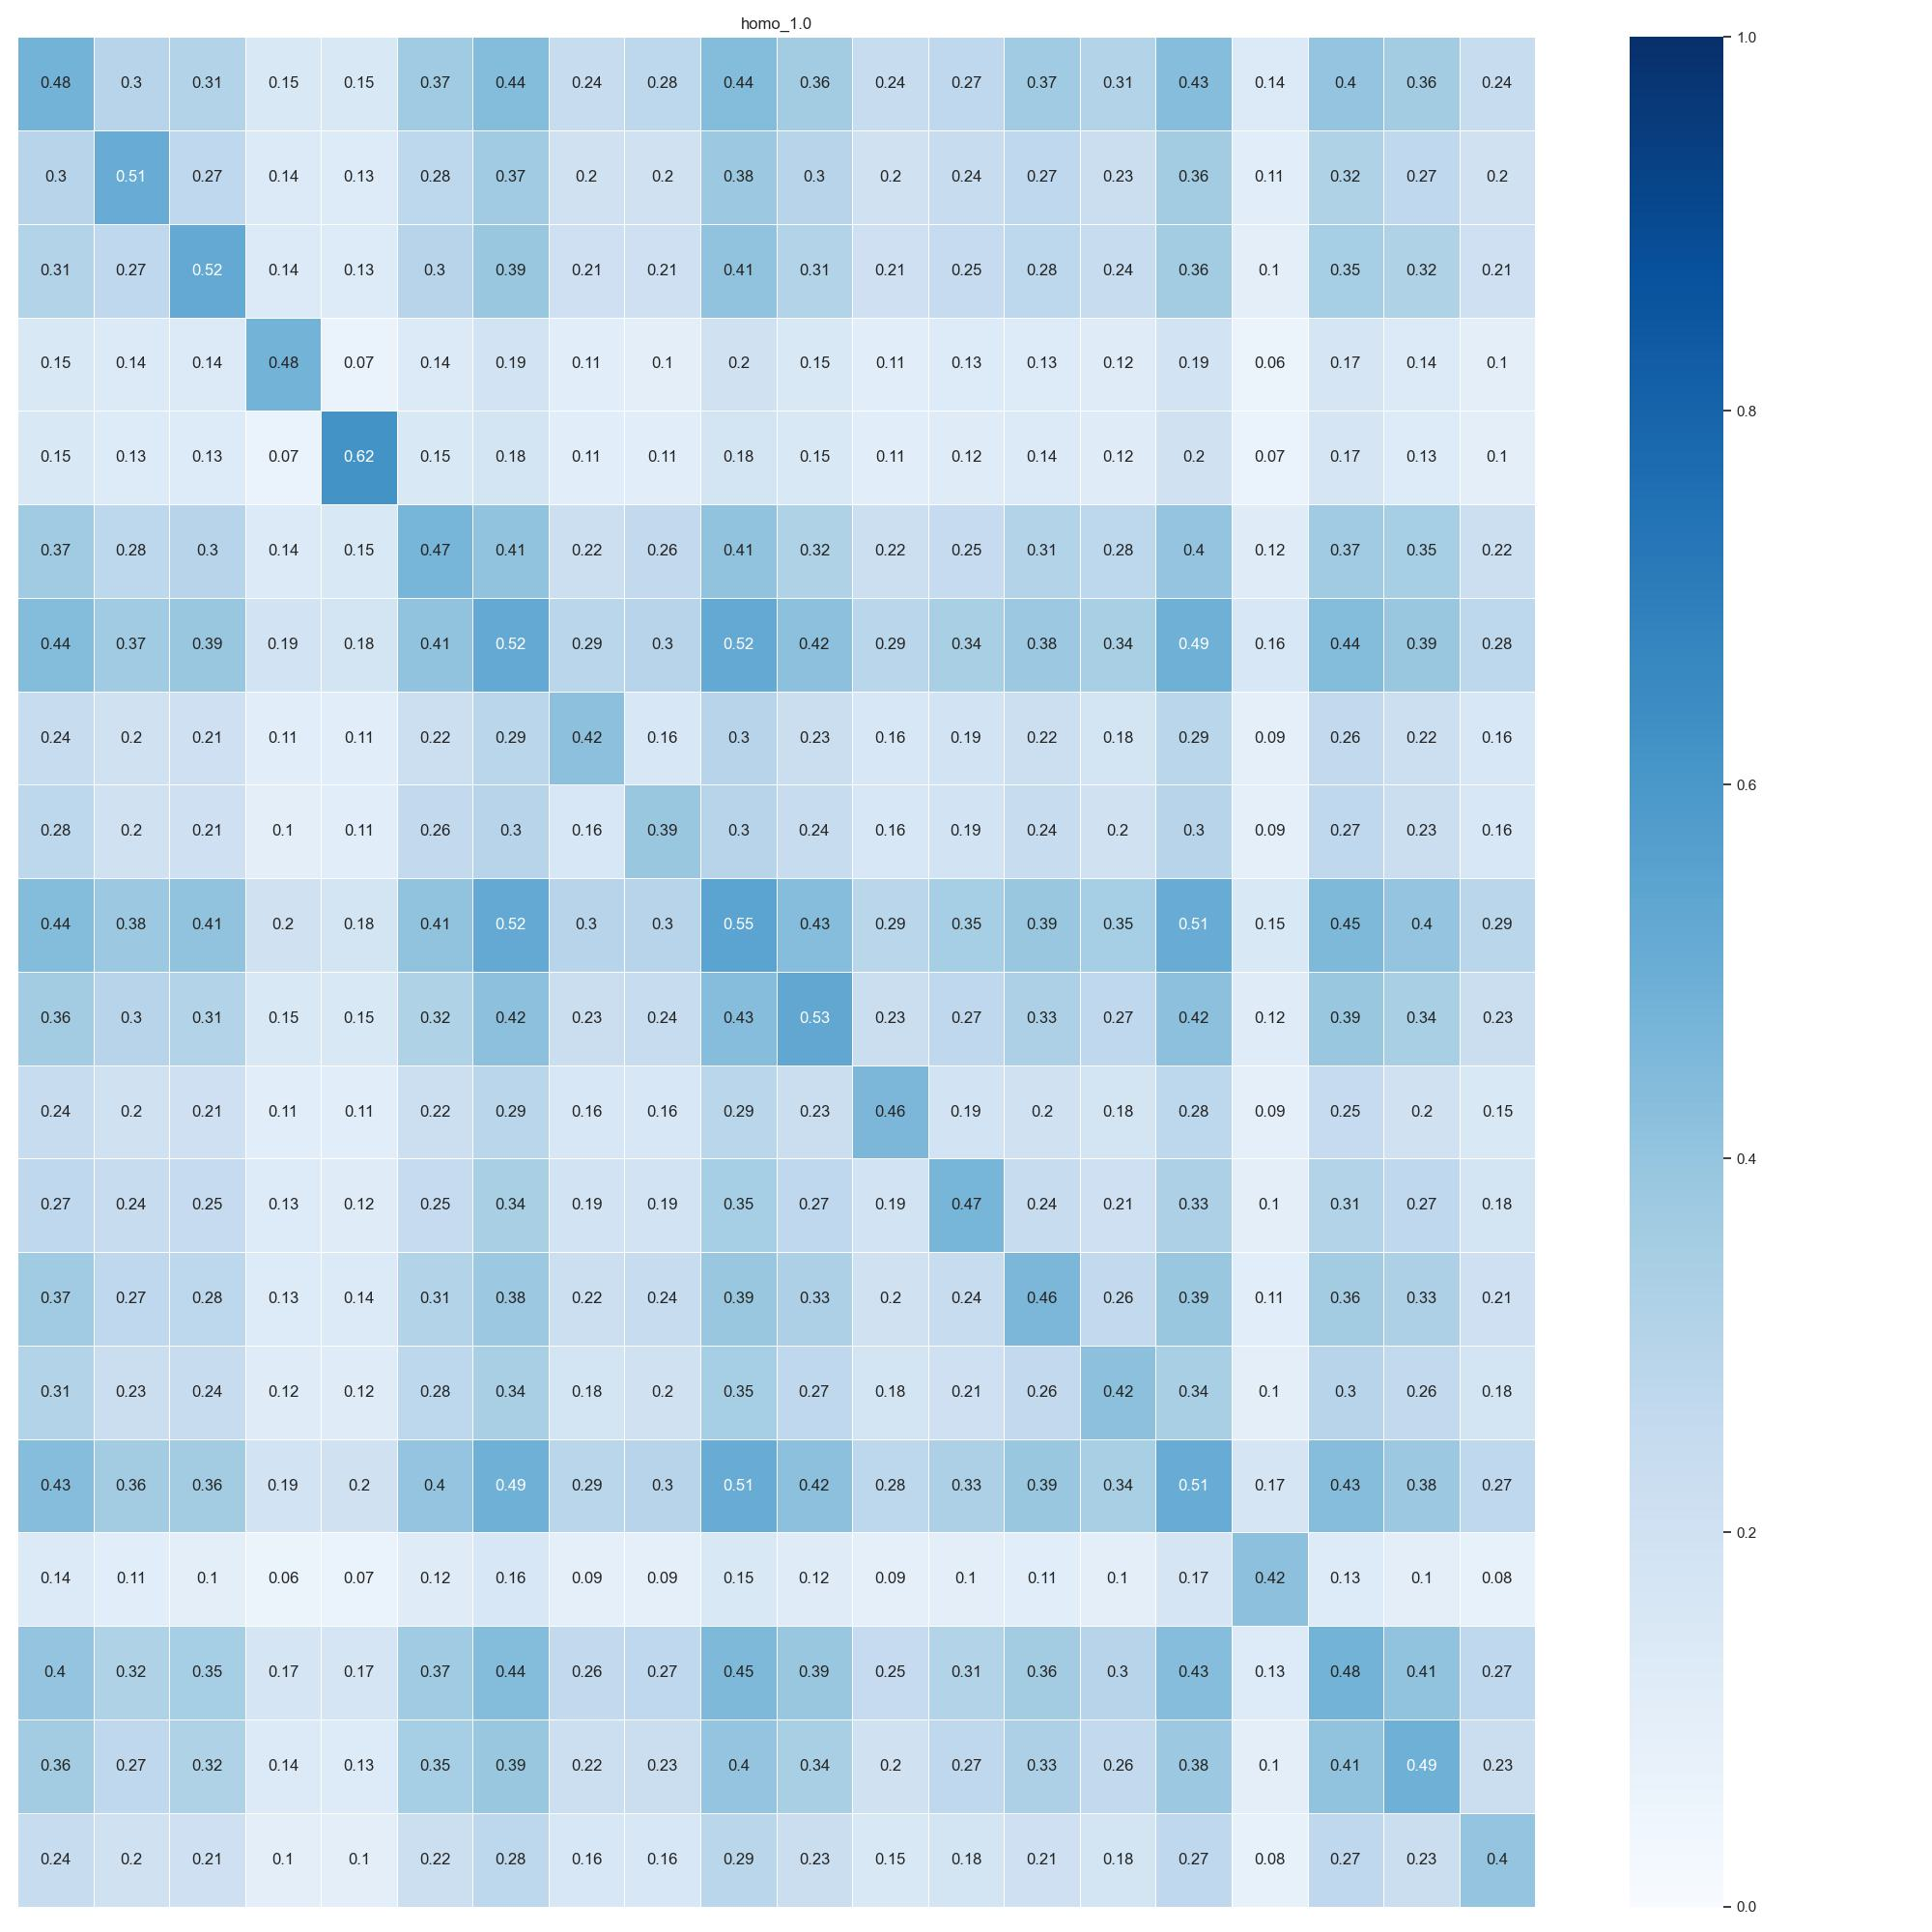}
         \caption{Cross-class Neighborhood Similarity in graph label homophily=1.0}
         \label{fig:ccns_1.0}
     \end{subfigure}
    \hfill
        \caption{Cross-class Neighborhood Similarity in hypersphere datasets with varying label homophily}
        \label{fig:ccns_hyper}
\end{figure}

\subsection{Hyperparameter Setting}
\label{hyperpara}
In this section, we summarize all the hyperparameters we used for the experiment section. The detailed setting is listed in Table \ref{Tab:hyper_mlp_gnn} and \ref{Tab:hyper_dw}.

More specifically, for \mlp and all GNN-based methods, we summarize the number of layers, the dimension of the hidden layer, the learning rate, the patience of the Earlystopping, the weight decay, and the number of neighbors we sample for the models that require sampling.

We use the same number of layers and the same hidden size for \mlp and the other GNN-based methods. The learning rate for the synthetic datasets in the varying feature quality and homophily experiments is $0.001$ instead of $0.01$ as in the other models because the performance of the \hgcn is further improved. We also use Earlystopping with the patience of $100$ epochs to train the models properly. For \graphsage, we sample $25$ and $20$ one and two hops away neighbors for aggregation. As other GNN-based baselines do not use the sampling method, the corresponding cells are filled with "No".

\begin{table}[!h]
\setlength{\tabcolsep}{3pt}
\caption{The hyperparameter setting for \mlp and GNN baselines in this work for all datasets}
\centering
\begin{tabular}{c|c|c|c|c}
\hline
         & MLP  & GCN, GAT, GraphSAGE    & H2GCN & GCN-LPA \\ \hline
Layers        & 2    & 2    & 2                                                                           & \begin{tabular}[c]{@{}c@{}}2 GCN\\ 5 LPA\end{tabular} \\ \hline
Hidden size            & 256  & 256                    & 256   & 256    \\ \hline
Learning rate & 0.01 & 0.01 & \begin{tabular}[c]{@{}c@{}}real-world: 0.01\\ synthetic: 0.001\end{tabular} & 0.01                                                  \\ \hline
Earlystopping patience & 100  & 100                    & 100   & 100     \\ \hline
Weight decay           & 5e-4 & 5e-4                   & 5e-4  & 1e-4    \\ \hline
Sample for aggregation & No   & GraphSAGE:{[}25, 10{]} & No    & No      \\ \hline
\end{tabular}

\label{Tab:hyper_mlp_gnn}
\end{table}

For the only random-walk-based method, we deploy the default setting for all the datasets in this work as \deepwalk already shows competitive performance. We perform $10$ random walks with the walk length of $10$ for each node to generate the sequence and use the window size of $5$ for the training pairs, the generated embedding size is $64$.
% Please add the following required packages to your document preamble:
% \usepackage{multirow}
\begin{table}[!h]
\setlength{\tabcolsep}{3pt}
\caption{The hyperparameter setting for \deepwalk in this work for all datasets}
\centering
\begin{tabular}{c|c|c|c|c}
\hline
\multirow{2}{*}{} & \multirow{2}{*}{Number of  walks} & \multirow{2}{*}{Walk length} & \multirow{2}{*}{Embedding size} & \multirow{2}{*}{Window size} \\
                                &                                   &                              &                                 &                             \\ \hline
DeepWalk                        & 10                                & 10                           & 64                              & 5                           \\ \hline
\end{tabular}
\label{Tab:hyper_dw}
\end{table}

\subsection {The experiment results and analysis}
\label{Experiment Results}
\subsubsection{Datasets}
We employ $7$ real-world datasets including \blog, \yelp, \ogb, \dblp, \pcg, \humloc, \eukloc, and $2$ sets of synthetic datasets with varying homophily and feature quality. For all datasets except \ogb, \humloc, and \eukloc we generate $3$ random training, validation, and test splits with $60$\%, $20$\%, and $20$\%  of the data. For \ogb, \humloc, and \eukloc we follow the predefined data splits from \citep{hu2020ogb}, \citep{shen2007hum} and \citep{chou2007euk} respectively. As \blog has no given node features, we use an identity matrix as the input feature matrix.

\begin{table}[h!] 
\setlength{\tabcolsep}{3pt}
 \caption{Dataset statistics. $|\mathcal{V}|$ and $|\mathcal{E}|$ denote the number of nodes and edges in the graph. $|\mathcal{F}|$ is the dimension of the node features. $clus$ and $r_{homo}$ denote the clustering coefficient and the label homophily. $C$ indicates the size of all labels in the graph. $\ell_{med}$, $\ell_{mean}$, and $\ell_{max}$ specify the median, mean, and max values corresponding to the number of labels of a node.  `$25$\%', `$50$\%', and `$75$\%' corresponds to the $25$th, $50$th, and $75$th percentiles of the sorted list of the number of labels for a node. "N.A." means the corresponding characteristic is not available in the graph.}
\small
\centering
 \begin{tabular}{lccccccccccccc}
\toprule
 \textsc{Dataset}             &  $|\mathcal{V}|$  & $|\mathcal{E}|$ &  $|\mathcal{F}|$    &  $clus$  &$r_{homo}$ & $C$ &$\ell_{med}$& $\ell_{mean}$  & $\ell_{max}$& $25$\% & $50$\% & $75$\%\\
\midrule
 \blog         & 10K    & 333K    &  N.A.      &0.46&0.10&39&1&1.40&11&1&1&2\\
 \yelp                & 716K   & 7.34M   &300&0.09&0.22&100&6&9.44&97&3&6&11\\
\ogb  &132K   &39M   &8&0.28&0.15&112&5&12.75&100&0&5&20\\
\dblp &28K &68K &300 &0.61 &0.76 &4  &1 &1.18 &4 &1 &1 &1 \\
 \hline
 \end{tabular}
 \label{tab:dataset}
\end{table}

\begin{table}[!h] 

\setlength{\tabcolsep}{3pt}
 \caption{Statistics for new datasets. The column notations are the same as in Table \ref{tab:dataset}.  }
\small
\centering
 \begin{tabular}{lccccccccccccc}
\toprule

\textsc{Dataset}             &  $|\mathcal{V}|$  & $|\mathcal{E}|$ &  $|\mathcal{F}|$    &  $clus$  &$r_{homo}$ & $C$ &$\ell_{med}$& $\ell_{mean}$  & $\ell_{max}$& $25$\% & $50$\% & $75$\%\\
  
\midrule
 \pcg   &3K   &37k   &32&0.34&0.17&15&1&1.93&12&1&1&2\\
 \humloc  &3.10k   &18K   &32&0.13&0.42&14&1&1.19&4&1&1&1\\
 \eukloc  &7.70K  &13K   &32&0.14&0.46&22&1&1.15&4&1&1&1\\
 \hline
 \end{tabular}
 \label{tab:newdataset}
\end{table}

\subsubsection{Compared Methods}
For a holistic evaluation we include four classes of compared methods (i) simple methods, which include Multilayer Perceptron (\mlp), which only uses node features and ignores the graph structure, and \deepwalk, which only uses graph structure and ignores the node features (ii) Convolutional neural networks based which employ convolutional operations to extract representations from node's local neighborhoods and merge them with label embeddings for the final classification. We choose \lanc as a baseline from this category, as previous works \citep{ZHOU2021115063, song2021semi} have shown its superior performance. (iii) graph neural networks including (a) \gcn, \gat, and \graphsage, which are known to perform well for graphs with high label homophily, and (b)\hgcn, which is designed to perform well both on homophilic and heterophilic graphs and  (iiii) \gcnlpa which combines label propagation and GCN for node classification. 

\subsubsection{Evaluation Metrics} We report the average micro- and macro-F1 score, macro-averaged AUC-ROC score, macro-averaged average precision score, and standard deviation over the three random splits. Due to space constraints, we report average precision (AP) in the main paper, and all detailed results are available in Tables \ref{tab:ex_res_realdatasets}, \ref{tab:ex_feat}, \ref{tab:ex_homo} in the Appendix \ref{Experiment Results}. Our choice of using AP over AUROC as the metric is also motivated in Appendix \ref{MetricDisscusion}.

We summarize the experimental results on the real-world datasets and the synthetic datasets in Table \ref{tab:ex_res_realdatasets}, Table \ref{tab:ex_feat}, and Table \ref{tab:ex_homo}, respectively. For better precision, we report the scores in percentages. Specifically, for the scores reported on \ogb, the difference between our results and those reported in the benchmark is because 1) we use $2$ layer \mlp without Node2Vec features. 2) We use Earlystopping with the patience of 100 epochs to prevent the models from being overtrained. 3) We use sampled local neighborhoods to have a consistent setting for all the datasets using \graphsage. The specific parameters we used are summarized in \ref{hyperpara}. Another pre-processing we did was to remove the isolated nodes in \pcg. The details are described in Appendix \ref{phenotypeDataDes}.
%[htbp]
\LTcapwidth=\textwidth
\begin{longtable}{ll cccc}
    % \centering
    \caption{Multi-label Node Classification results on real-world datasets. The results of \blog, \yelp, \pcg, and \dblp are the mean of three random splits with $60$\% for train-, $20$\% validation and $20$\% test dataset, while the results of \ogb, \humloc, \eukloc are reported with the built-in split. }\\
   % \small {
   % \SetTblrInner{rowsep=0pt}
   % \setlength\extrarowheight{-3pt}
    % \begin{NiceTabular}{ll cccc}
\toprule
{\textbf{\textsc{Dataset}}} & {\textbf{\textsc{Method}}} & 
     \textsc{Micro-F1} &   \textsc{Macro-F1} &   \textsc{AUC-ROC} & \textsc{AP}\\  
     \midrule
     \endhead
     
 \multirow{8}{*}{\rotcell{\blog}}& {\mlp} &$17.11 \pm 0.64$
 & $2.49 \pm 0.18$    & $50.30 \pm 1.04$ & $4.25 \pm 0.63$    \\ 
 & \deepwalk & $ \bf{35.59 \pm 0.21}$
  & $ \bf{19.74  \pm 0.54}$  & $\bf{73.20 \pm 0.58}$   & $\bf{18.55 \pm 0.17}$   \\
  &\lanc & $ 13.95\pm 2.02$ 
& $ 4.55\pm 0.82$     & $ 52.34\pm 0.91$    & $\underline{5.03 \pm 0.07}$  \\
 &{\gcn} & $16.69 \pm 0.47$
 & $ \underline{2.63\pm 0.08}$    & $47.85 \pm 0.06$   & $3.69 \pm 0.04$   \\
 & {\gat} & $ \underline{17.22\pm 0.52}$
 & $2.48 \pm 0.08$    & $50.88 \pm 1.45$   & $4.05\pm0.09$   \\
 & {\graphsage} & $ 16.18\pm0.31 $
 & $ 2.38\pm 0.27$    & $ \underline{52.73\pm 0.82}$  &  $4.50\pm0.12$  \\
 & {\hgcn} & $16.86 \pm 0.34$ 
& $ 2.60\pm 0.16$     & $49.83 \pm 1.08$    & $3.92 \pm 0.05$   \\
 & {\gcnlpa} & $ 17.15\pm0.68 $ 
& $ 2.55\pm0.19 $     & $51.35 \pm 0.67$    & $ 4.33\pm 0.31$   \\
 
 \midrule

 \multirow{8}{*}{\rotcell{\yelp}}& {\mlp} & $ 26.04\pm 0.09$
 & $ 18.55\pm 0.20$    & $ 50.17\pm 0.01$   & $ 9.58\pm 0.01$   \\ 
 & {\deepwalk} &$49.78 \pm 0.07$ 
 &$24.98 \pm 0.04$     & $50.67 \pm 0.08$   & $9.60 \pm 0.02$   \\
  &\lanc & $-$ & $-$     & $-$    & $-$   \\
 &{\gcn} & $52.21 \pm 0.07$
 &  $ 27.60\pm 0.04$   & $53.81 \pm 0.13$   &  $ 13.14\pm 0.06$  \\
 & {\gat} & $51.24 \pm 0.08$
 & $26.66 \pm 0.06$    & $67.80 \pm 0.05$   &  $15.00 \pm 0.07$  \\
 & {\graphsage} & $\bf{56.06 \pm 0.10}$
 & $\bf{31.26 \pm 0.10}$    & $\bf{81.05 \pm 0.25}$   & $\bf{25.09 \pm 0.31}$   \\
 & {\hgcn} & $ \underline{54.12\pm 0.01}$ 
 &  $ \underline{30.52\pm 0.11}$    &  $ \underline{75.25\pm 0.46}$   &  $ \underline{22.57\pm 0.51}$   \\
  & {\gcnlpa} & $ 50.31\pm0.29 $ 
& $25.68\pm0.43 $     & $61.09 \pm2.27 $    & $ 11.62\pm0.74 $   \\ 
 
 \midrule

 \multirow{8}{*}{\rotcell{\ogb}}& {\mlp} & $2.55$
 & $2.40$     & $54.05$   & $2.59$    \\ 
 & {\deepwalk} & $\bf{2.88}$
 & $\bf{2.75}$     &$\underline{68.75}$    & $4.41$   \\
    &\lanc & $2.35$ 
& $2.21$     & $68.03$    & $\underline{4.48}$   \\
 &{\gcn} & $\underline{2.77}$ 
 & $\underline{2.63}$    & $\bf{71.48}$   & $\bf{5.36}$    \\
  & {\gat} & $ 2.55$
 &  $ 2.40$   &  $ 50.64$   & $ 2.14$    \\
 & {\graphsage} & $2.59$ 
 & $2.43$    & $55.83$   &  $2.68$  \\
 & {\hgcn} & $2.55 $ 
  &  $ 2.39 $   & $ 62.75$    & $ 3.61$    \\
   & {\gcnlpa} & $2.56$ 
& $2.41 $     & $ 53.22 $    & $2.33 $   \\
 
 \midrule
 %-----------------------------------------------------
 \multirow{8}{*}{\rotcell{\dblp}}& {\mlp} &$ 42.14\pm 0.27$
 &$ 32.04\pm0.65 $   &$ 54.47\pm0.07 $   &$ 34.97\pm0.14 $    \\ 
& {\deepwalk} &$ 63.27\pm0.34 $
 &$ 59.11\pm 0.36$   &$74.81 \pm0.16 $   &$ 58.49\pm 0.25$    \\ 
 & {\lanc} &$ 81.93\pm0.29 $
 &$ 80.39\pm0.42 $   &$ 91.76\pm0.36 $   &$ 83.55\pm 0.98$    \\ 
 & {\gcn} &$ \bf{87.03\pm0.20} $
 &$ \bf{85.80\pm0.38} $   &$ \underline{94.15\pm0.16} $   &$ \bf{89.27\pm 0.24}$    \\ 
 & {\gat} &$ 83.06\pm0.17 $
 &$ 81.26\pm 0.14$   &$ 92.57\pm0.07 $   &$ 82.93\pm 0.16$    \\ 
 & {\graphsage} &$ \underline{85.22\pm 0.23}$
 &$ \underline{83.89\pm 0.21}$   &$ \bf{94.32\pm 0.02}$   &$ \underline{86.84\pm 0.18}$    \\ 
 & {\hgcn} &$ 83.99\pm 0.92$
 &$ 82.56\pm 0.86$   &$ 92.14\pm 0.57$   &$ 85.82\pm 0.64$    \\ 
 & {\gcnlpa} &$ 82.88\pm0.31 $
 &$ 81.31\pm0.34 $   &$ 90.17\pm 0.43$   &$ 80.07\pm1.24 $    \\ 

 \midrule
  %-----------------------------------------------------
 \multirow{8}{*}{\rotcell{\pcg}}& {\mlp} &$38.04 \pm 1.20$
 &$18.03  \pm 1.29$   &$51.07 \pm 0.63$   &$14.78 \pm 0.60$    \\ 
 & {\deepwalk} &$ \bf{42.26 \pm 1.37}$
 &$ \bf{31.49 \pm 0.90}$   & $ \bf{63.58 \pm 0.87}$   & $\bf{22.86 \pm 1.00}$    \\
   &\lanc & $ 36.28\pm 0.34$ 
& $20.50\pm1.15 $     & $ 56.58\pm 0.69$    & $ 18.53\pm 1.14$   \\
 &{\gcn} &$ \underline{41.46 \pm 1.21}$
 &$\underline{25.59 \pm 0.92}$    &$\underline{59.54  \pm 0.82}$  & $\underline{21.03 \pm 0.34}$   \\
  & {\gat} & $36.91 \pm 1.75$ 
 & $19.24 \pm 0.75 $    &$56.33 \pm 4.64 $   & $16.75 \pm 2.17$    \\
 & {\graphsage} &$38.89 \pm 1.17$
 &$24.44 \pm 1.74$  & $58.57 \pm 0.08$   &  $18.45 \pm 0.29$  \\
 & {\hgcn} &$39.05 \pm 0.99$
 & $24.38  \pm 2.17$   &$58.10  \pm 0.14$  & $19.19 \pm 0.49$    \\
   & {\gcnlpa} & $ 39.57\pm1.12 $ 
& $22.90\pm 1.33$     & $ 54.74\pm0.95 $    & $ 16.71\pm 0.14$   \\

 \midrule

 \multirow{8}{*}{\rotcell{\humloc}}& {\mlp} & $42.12$
 & $18.04$    & $66.04$   & $16.95$   \\ 
 & {\deepwalk} & $45.26$
 &  $\underline{23.30}$   & $65.67$   &  $18.58$  \\
  &\lanc & $39.25 $ 
& $11.51$     & $ 59.65 $    & $ 13.24 $   \\
 &{\gcn} & $\bf{51.67}$ & $\bf{25.57}$    & $67.28$   &  $\bf{25.15}$  \\
 & {\gat} & $47.10$
 & $17.49$    &  $\bf{72.47}$  &  $\underline{23.75}$  \\
 & {\graphsage} & $\underline{48.05}$
 &  $21.22$   &  $\underline{70.30}$  &  $23.42$  \\
 & {\hgcn} & $45.39$
 & $18.35$    &  $64.31$  &  $17.23$  \\
   & {\gcnlpa} & $45.73 $ 
& $18.15 $     & $ 62.40 $    & $ 14.96 $   \\
 \midrule

 \multirow{8}{*}{\rotcell{\eukloc}}& {\mlp} & $43.58$
 &  $11.13$   &  $66.83$  &  $12.00$  \\ 
 & {\deepwalk} & $34.67$
 &  $6.74$   &  $56.12$  & $7.58$   \\
 &\lanc & $ 36.08 $ 
& $4.55$     & $ 51.13$    & $ 6.16$   \\
 &{\gcn} & $\bf{45.86}$
 &  $\bf{12.27}$   &  $\underline{70.53}$  & $\bf{15.15}$   \\
 & {\gat} & $41.58$
 & $6.76$    &  $\bf{71.65}$  &  $\underline{13.59}$  \\
 & {\graphsage} & $44.65$
 &  $\underline{11.96}$   &  $69.04$  & $12.44$   \\
 & {\hgcn} & $\underline{44.93}$
 &  $11.80 $  & $69.45$   &  $13.35$\\
   & {\gcnlpa} & $ 36.72 $ 
& $5.93 $     & $ 56.65 $    & $ 7.45 $   \\

\bottomrule
% \end{NiceTabular}
    % }
    \label{tab:ex_res_realdatasets}
\end{longtable}

\begin{table*}[htbp]
    
    \caption{Multi-label Node Classification results on Synthetic dataset with varying feature quality. All results are the mean of three random splits. The Ratios of the relevant and the irrelevant features are $[0, 0.2, 0.5, 0.8, 1.0]$.}
    \small{
    \centering
    \begin{NiceTabular}{ll cccc}
\toprule
{\textbf{\textsc{Feature Ratios}}} & {\textbf{\textsc{Method}}} & 
     \textsc{Micro-F1} &   \textsc{Macro-F1} &   \textsc{AUC-ROC} & \textsc{AP}\\
 \multirow{8}{*}{\rotcell{0}}& {\mlp} &$ 67.05 \pm 0.91$
 & $ 25.15\pm 0.89$   & $ 50.99\pm 1.11$  &  $ 17.17\pm 0.42$  \\ 
 & \deepwalk & $ \bf{86.22\pm 0.39}$
  & $ \bf{47.80 \pm 0.31}$   & $ \bf{84.15 \pm 0.56}$  & $ \bf{48.70\pm 0.51}$   \\
   &\lanc &$ 69.67\pm 0.26 $
&$ 26.68\pm 1.16$    &$  75.36\pm 1.17$  &  $ 33.68\pm 0.88$  \\
 &{\gcn} &$ 67.09\pm 0.95$
 & $  25.12\pm 1.09$   & $  77.17\pm 0.92$  & $ 31.27\pm0.66 $   \\
 & {\gat} &$  66.67 \pm 0.71$
 &$  25.09\pm 1.24  $  &$61.96 \pm	3.97 $   & $ 31.10 	\pm 3.17 $   \\
 & {\graphsage} & $ 67.90 \pm 1.40 $ & $  25.87 \pm	1.51 $
 & $ 66.47 \pm 0.31 $    & $ 30.01 \pm	0.71 $   \\
 & {\hgcn} &$\underline{ 71.12\pm1.26 } $
&$ \underline{27.45\pm 1.18} $    &$ \underline{80.83 \pm 0.98} $  &  $ \underline{37.64\pm 1.72}$  \\
 & {\gcnlpa} &$ 70.26\pm2.00  $
&$ 26.70\pm1.47 $    &$ 70.58 \pm 2.04 $  &  $ 33.65\pm 2.61$  \\

 \midrule

 \multirow{8}{*}{\rotcell{0.2}}& {\mlp} &$68.37 \pm 0.55$
 &$ 26.61\pm 0.47$    &$54.47 \pm 0.19$   & $ 18.70\pm 0.69 $   \\ 
 & {\deepwalk} & $ \bf{86.22\pm 0.39}$
 &$ \bf{47.80\pm 0.31}$   &$ \bf{84.15\pm 0.56} $  & $\bf{48.70\pm0.51} $\\
 &\lanc &$ 70.84\pm1.75  $
&$ 27.62\pm0.74 $    &$ 74.42 \pm 2.02$  &  $ 34.24\pm 1.42$  \\
 &{\gcn} &$ 67.42 \pm 1.07$ 
 &$ 25.31\pm 1.09 $  &$ 77.47 \pm 0.87$   &  $31.59\pm0.63$  \\
 & {\gat} &$ 67.07\pm 1.07$
 &$ 25.03\pm 1.16$    &$ 64.55\pm0.60 $  & $33.90\pm0.30$   \\
 & {\graphsage} & $ 70.14\pm 0.60$
 & $ 27.99\pm1.07  $    & $ 69.44\pm 1.09$  &  $ 32.84\pm0.79 $  \\
 & {\hgcn} & $ \underline{73.21\pm 1.07}$
 & $ \underline{28.85\pm 1.23}$   & $ \underline{ 81.78\pm1.24} $  &  $ \underline{40.12\pm4.24}  $  \\
  & {\gcnlpa} &$ 69.67 \pm 1.67 $
&$ 26.14\pm 1.53$    &$ 71.02\pm 1.71$  &  $ 33.33\pm 1.31$  \\
 
 \midrule

 \multirow{8}{*}{\rotcell{0.5}}& {\mlp} &$ 68.83 \pm	0.78  $ 
 &$ 27.57 \pm	1.10 $   & $61.63 \pm	0.74  $  &   $21.95 \pm0.40 $ \\ 
 & {\deepwalk} & $ \bf{86.22 \pm	0.39 } $
 &$\bf{47.80 \pm	0.31 }$   &$\underline{84.15 \pm	0.56 }$  & $\bf{48.70 \pm	0.51} $\\
  &\lanc &$73.21 \pm 2.79$
&$ 30.02\pm 2.01$    &$ 77.05\pm 1.16$  &  $ 36.45\pm 1.30$  \\
 &{\gcn} &$67.55 \pm	1.08$
 & $ 25.39 \pm	1.08  $   & $ 77.25 \pm	0.85 $  & $ 31.14 \pm	0.61$    \\
  & {\gat} & $67.76 \pm	1.75 $
 &$ 25.49 \pm	1.46$  &$ 64.40 	\pm1.64  $ & $32.92 	\pm0.88 $   \\
 & {\graphsage} &$74.70 	\pm0.49  $
 &$ 31.25 \pm	0.89$   & $ 76.24 \pm	0.47 $  & $ 37.65 \pm	0.65  $   \\
 & {\hgcn} &$ \underline{76.16 \pm	0.47} $
 &$ \underline{32.85 \pm 0.28 }$   &$  \bf{84.96 	\pm 0.55}$  &  $ \underline{42.70 \pm	0.27} $  \\
  & {\gcnlpa} &$ 72.11 \pm	1.89$
&$ 27.80 \pm	0.77$    &$ 74.39 \pm	1.26 $  &  $ 36.84 \pm	1.02 $  \\

 \midrule

 \multirow{8}{*}{\rotcell{0.8}}& {\mlp} &$  70.17 \pm	0.81  $
 &$  29.37 	\pm0.99 $   & $69.53 \pm	0.46 $   & $27.65 \pm	0.77 $ \\ 
 & {\deepwalk}  &$\bf 86.22 \pm	0.39  $
 &$ \bf 47.80 \pm	0.31 $   &$\underline{84.15 \pm	0.56 }$  & $ \bf 48.70 \pm	0.51  $\\
 &\lanc &$ 72.67\pm 3.56$
&$ 29.67\pm3.13 $    &$ 74.73\pm1.07 $  &  $ 35.32\pm 2.06$  \\
 &{\gcn} &$69.56 \pm	1.14  $ 
 &$   25.79 	\pm1.14 $    &$  77.03 \pm	0.99 $  &$ 30.10 \pm	0.71 $  \\
  & {\gat} &$ 67.93 \pm	0.75  $
 &$ 25.40 	\pm 1.17 $   &$ 66.41 \pm	3.55  $  &  $ 33.78 \pm	0.96 $  \\
 & {\graphsage} &$ 75.66 \pm	0.51 $
 &$ 32.39 	\pm 1.50  $   &$78.31 	\pm 0.49  $   & $39.25 \pm	0.86 $   \\
 & {\hgcn} &$ \underline{78.68 \pm	0.38} $
 &$ \underline{36.17 	\pm0.56} $    &$ \bf86.01\pm 	0.64  $  &  $\underline{44.21\pm 	0.31}$  \\
   & {\gcnlpa} &$ 72.62 	\pm1.46 $
&$27.74 \pm	0.67$    &$ 73.99 \pm	1.06$  &  $36.28 \pm	1.57  $  \\
 
 \midrule	
 
 \multirow{8}{*}{\rotcell{1.0}}& {\mlp} & $72.90 \pm 0.27$ & $ 31.52\pm 0.52$    &$ 75.23\pm 0.63$   & $ 34.29\pm 0.07$ \\
 & {\deepwalk}  & $ \bf86.22\pm0.39  $
 & $ \bf47.80\pm0.31 $    & $\underline{ 84.15\pm 0.56}$  &  $ \bf48.70\pm 0.51$\\
 &\lanc &$ 74.13\pm 1.61$
&$ 30.38\pm 1.29$    &$ 75.26\pm 0.93$  &  $ 37.47\pm 0.27$  \\
 &{\gcn} & $ 70.74 \pm0.80 $
 &  $ 26.57\pm 0.97$  &  $ 79.22 \pm 0.82$  & $ 33.70\pm0.79$ \\
  & {\gat} & $ 70.22\pm 1.27$
 & $ 26.35\pm 0.93$  &$ 66.52\pm1.03 $  & $ 36.01\pm 0.72$   \\
 & {\graphsage} & $ 78.71\pm0.59  $
 & $ 35.77 \pm1.40 $   & $ 80.77 \pm 0.17$  &  $ 43.05  \pm 	0.22$ \\
 & {\hgcn} & $\underline{79.97 \pm	0.19 }  $
 & $ \underline{38.73 \pm	0.91 }$   &$ \bf87.09 \pm 	0.12$ & $\underline{46.71  \pm	0.37 } $   \\
   & {\gcnlpa} &$ 76.28\pm1.27  $
&$31.91\pm1.07 $    &$ 76.38\pm 0.36$  &  $39.10\pm 2.03 $  \\
 
\bottomrule
\end{NiceTabular}
    }
    \label{tab:ex_feat}
\end{table*}

\begin{table*}[htbp]
    
    \caption{Multi-label Node Classification results on Synthetic dataset with varying label homophily. All results are the mean of three random splits. The label homophiles (rounded up) are $[0.2, 0.4, 0.6, 0.8, 1.0]$}
    \small{
    \centering
    \begin{NiceTabular}{ll cccc}
\toprule
{\textbf{\textsc{Label Homophily}}} & {\textbf{\textsc{Method}}} &\textsc{Micro-F1} &\textsc{Macro-F1} &   \textsc{AUC-ROC} & \textsc{AP}\\
 \multirow{8}{*}{\rotcell{0.2}}& {\mlp} &$ 72.90 \pm 0.27 $ &$ \underline{31.52 \pm 0.52} $   &$ \bf 75.23 \pm 0.63 $  &$ \bf{34.29 \pm 0.07 }$ \\ 
 & {\deepwalk} &$ 66.62 \pm 0.62 $  &$ 26.02 \pm 0.55 $ &$ 52.19 \pm 0.91 $ &$ 18.07 \pm 0.71 $\\
   &\lanc & $ 67.05\pm 0.92$ 
& $25.12\pm2.20$     & $54.49\pm0.53 $    & $ 18.95\pm 0.43$   \\
 &{\gcn} &$ 67.28 \pm 0.67 $ &$ 25.21 \pm 1.04 $ &$ 66.59 \pm 0.58 $ &$ 26.06 \pm 1.07 $ \\
 & {\gat}&$ 65.09 \pm 0.89 $ &$ 24.61 \pm 1.41 $ &$ 51.43 \pm 0.33 $ &$ 17.05 \pm 0.36 $ \\
 & {\graphsage} &$ \underline{73.57 \pm 0.20}$ &$ 31.22 \pm 0.65 $ &$ 71.72 \pm 0.30 $ &$ 28.94 \pm 1.09 $ \\
 & {\hgcn} &$ \bf73.80 \pm 0.59 $ &$ \bf 31.86 \pm 0.89 $ &$ \underline{73.24 \pm 0.08} $ &$ \underline{29.69 \pm 0.53} $ \\
 & {\gcnlpa}&$ 67.02 \pm 0.89 $ &$ 25.24 \pm 1.31 $ &$ 49.92 \pm 0.93 $ &$ 17.02 \pm 0.31 $  \\
 \midrule
 
 \multirow{8}{*}{\rotcell{0.4}} & {\mlp} &$ 72.90 \pm 0.27$ &$ 31.52 \pm 0.52 $ &$ 75.23 \pm 0.63 $ &$34.29 \pm 0.07 $\\ 
& {\deepwalk} &$ \bf 88.79 \pm 0.20 $ &$ \bf 54.74 \pm 1.73 $ &$ \underline{85.74 \pm 0.33} $ &$ \bf 52.15 \pm 1.41 $\\ 
 &\lanc & $ 75.16\pm 0.77$ 
& $33.69\pm0.94$     & $ 76.53\pm0.86 $    & $ 37.99\pm 0.74$   \\
&{\gcn}&$ 72.16 \pm 1.70 $ &$ 26.95 \pm 1.18 $ &$ 80.19 \pm 0.75 $ &$ 34.29 \pm 
0.88 $\\
& {\gat} &$ 71.50 \pm 1.30 $ &$ 27.58 \pm 1.11 $ &$ 69.96 \pm 1.69 $ &$ 35.86 \pm 0.59 $ \\
& {\graphsage} &$ 79.09 \pm 0.33 $ &$ 36.05 \pm 1.56 $ &$ 81.00 \pm 0.35 $ &$ 42.57 \pm 0.49 $ \\ 
& {\hgcn} &$ \underline{81.30 \pm 0.25} $ &$ \underline{40.54 \pm 0.74} $ &$ \bf 87.91 \pm 0.04 $ &$ \underline{48.36 \pm 0.44} $\\
& {\gcnlpa}&$ 78.11 \pm 1.38 $ &$ 32.71 \pm 1.47 $ &$ 78.00 \pm 0.70 $ &$ 40.80 \pm 0.20 $\\

\midrule

 \multirow{8}{*}{\rotcell{0.6}} & {\mlp}  &$ 72.90 \pm 0.27 $
&$ 31.52 \pm 0.52 $
&$ 75.23 \pm 0.63 $
&$ 34.29 \pm 0.07 $\\ 
 & {\deepwalk} &$ \bf 95.94 \pm 0.05 $
&$ \bf 82.58 \pm 0.19 $
&$ \bf 95.32 \pm 0.80 $
&$ \bf 81.34 \pm 0.95 $\\
&\lanc & $ 80.36\pm 1.81$ 
& $39.65\pm3.14$     & $81.85 \pm 2.66$    & $ 43.42\pm3.61 $   \\
 &{\gcn} &$ 75.47 \pm 0.46 $
&$ 29.43 \pm 0.43 $
&$ 84.08 \pm 0.72 $
&$ 38.78 \pm 0.33 $ \\
  & {\gat} &$ 75.13 \pm 0.39 $
&$ 29.26 \pm 0.56 $
&$ 72.85 \pm 0.79 $
&$ 39.01 \pm 0.23 $
 \\
 & {\graphsage} &$ 82.46 \pm 0.67 $
&$ 40.46 \pm 1.67 $
&$ 83.24 \pm 0.89 $
&$ 45.79 \pm 0.91 $ \\
 & {\hgcn}&$ 83.40 \pm 1.94 $
&$ 44.32 \pm 1.59 $
&$ \underline{89.98 \pm 0.86} $
&$ \underline{51.19 \pm 1.92} $
\\
  & {\gcnlpa} &$ \underline{85.45 \pm 2.42} $
&$ \underline{47.67 \pm 4.72} $
&$ 83.96 \pm 2.22 $
&$ 49.54 \pm 3.54 $\\

 \midrule
 \multirow{8}{*}{\rotcell{0.8}}& {\mlp} &$ 72.90 \pm 0.27 $
&$ 31.52 \pm 0.52 $
&$ 75.23 \pm 0.63 $
&$ 34.29 \pm 0.07 $
\\ 
 & {\deepwalk}  &$ \bf{ 96.53 \pm 0.61} $
&$ \bf{89.25 \pm 1.96} $
&$ \bf{95.81 \pm 0.47} $
&$ \bf{86.93 \pm 1.92} $\\
 &\lanc & $ 79.35\pm0.97 $ 
& $46.03\pm2.24$     & $ 87.75\pm 0.60$    & $ 48.10\pm1.17 $   \\
 &{\gcn}&$ 80.72 \pm 0.55 $
&$ 36.60 \pm 1.31 $
&$ 86.82 \pm 0.62 $
&$ 44.98 \pm 0.40 $\\
  & {\gat}&$ 77.35 \pm 0.49 $
&$ 31.63 \pm 1.10 $
&$ 83.10 \pm 0.69 $
&$ 42.82 \pm 0.86 $ \\
 & {\graphsage} &$ 84.22 \pm 0.38 $
&$ 48.16 \pm 1.42 $
&$ 87.37 \pm 0.34 $
&$ 53.34 \pm 0.84 $\\
 & {\hgcn} &$ 86.00 \pm 2.63 $
&$ 55.85 \pm 4.92 $
&$ \underline{91.61 \pm 1.64} $
&$ 57.17 \pm 2.57 $\\
   & {\gcnlpa} &$ \underline{88.96 \pm 0.68} $
&$\underline{ 64.09 \pm 4.18 }$
&$ 89.53 \pm 1.07 $
&$ \underline{60.44 \pm 4.41} $\\
% \midrule

 \midrule

 \multirow{8}{*}{\rotcell{1.0}}& {\mlp} &$ 72.90 \pm 0.27 $
&$ 31.52 \pm 0.52 $
&$ 75.23 \pm 0.63 $
&$ 34.29 \pm 0.07 $\\
 & {\deepwalk} &$ 80.25 \pm 0.11 $
&$ \underline{62.80 \pm 0.46} $
&$ 83.83 \pm 1.08 $
&$ 55.16 \pm 0.67 $\\
 &\lanc & $ 83.37\pm 0.96$ 
& $60.77\pm3.51$     & $ \underline{92.53\pm 1.27}$    & $ \underline{62.85\pm 3.01}$   \\
 &{\gcn} &$ 81.61 \pm 0.25 $
&$ 42.19 \pm 0.45 $
&$ 86.48 \pm 0.31 $
&$ 49.32 \pm 0.92 $
\\
  & {\gat} &$ 79.37 \pm 0.64 $
&$ 34.67 \pm 1.87 $
&$ 87.20 \pm 2.15 $
&$ 43.90 \pm 2.90 $
  \\
 & {\graphsage} &$ 82.15 \pm 0.49 $
&$ 46.06 \pm 0.99 $
&$ 89.73 \pm 0.45 $
&$ 55.25 \pm 0.42 $ \\
 & {\hgcn} &$ \bf{91.59 \pm 1.74} $
&$ \bf{76.09 \pm 5.96} $
&$ \bf{93.94 \pm 1.03} $
&$ \bf{65.20 \pm 5.71} $  \\
  & {\gcnlpa} &$ \underline{86.92 \pm 1.13} $
&$ 60.71 \pm 3.01 $
&$ 90.75 \pm 0.46 $
&$ 58.28 \pm 3.02 $
\\
\\
\bottomrule
\end{NiceTabular}
    }
    \label{tab:ex_homo}
\end{table*}

\subsection{Challenge of the Evaluation Metrics}
\label{MetricDisscusion}
The Area under the ROC curve (AUC) and the Area under the Precision-Recall curve (AUPR) are two widely accepted non-parametric measurement scores used by existing works. Nevertheless, as discussed in~\citep{yang2015evaluating}, the AUC score is sometimes misleading for highly imbalanced datasets like those in our work. In addition, AUPR might lead to over-estimation of the models' performance when the number of thresholds (or unique prediction values) is limited \citep{dong2020towards}. For such reasons, as suggested in~\citep{dong2020towards}, we instead use the Average Precision (AP) score as our primary evaluation metric. Following previous works, we also report the F1 score. As it is a threshold-based metric we emphasize that it might be biased when the benchmarked models have different prediction score ranges.

\subsection{Cross-class Neighborhood Similarity Plots}
In this section, we put the heat maps of the cross-class neighborhood similarity for all the datasets used in this work. We use color coding, where a darker shade in the cell indicates a stronger cross-class neighborhood similarity.

\begin{figure}
     \centering
        \includegraphics[width=\linewidth]{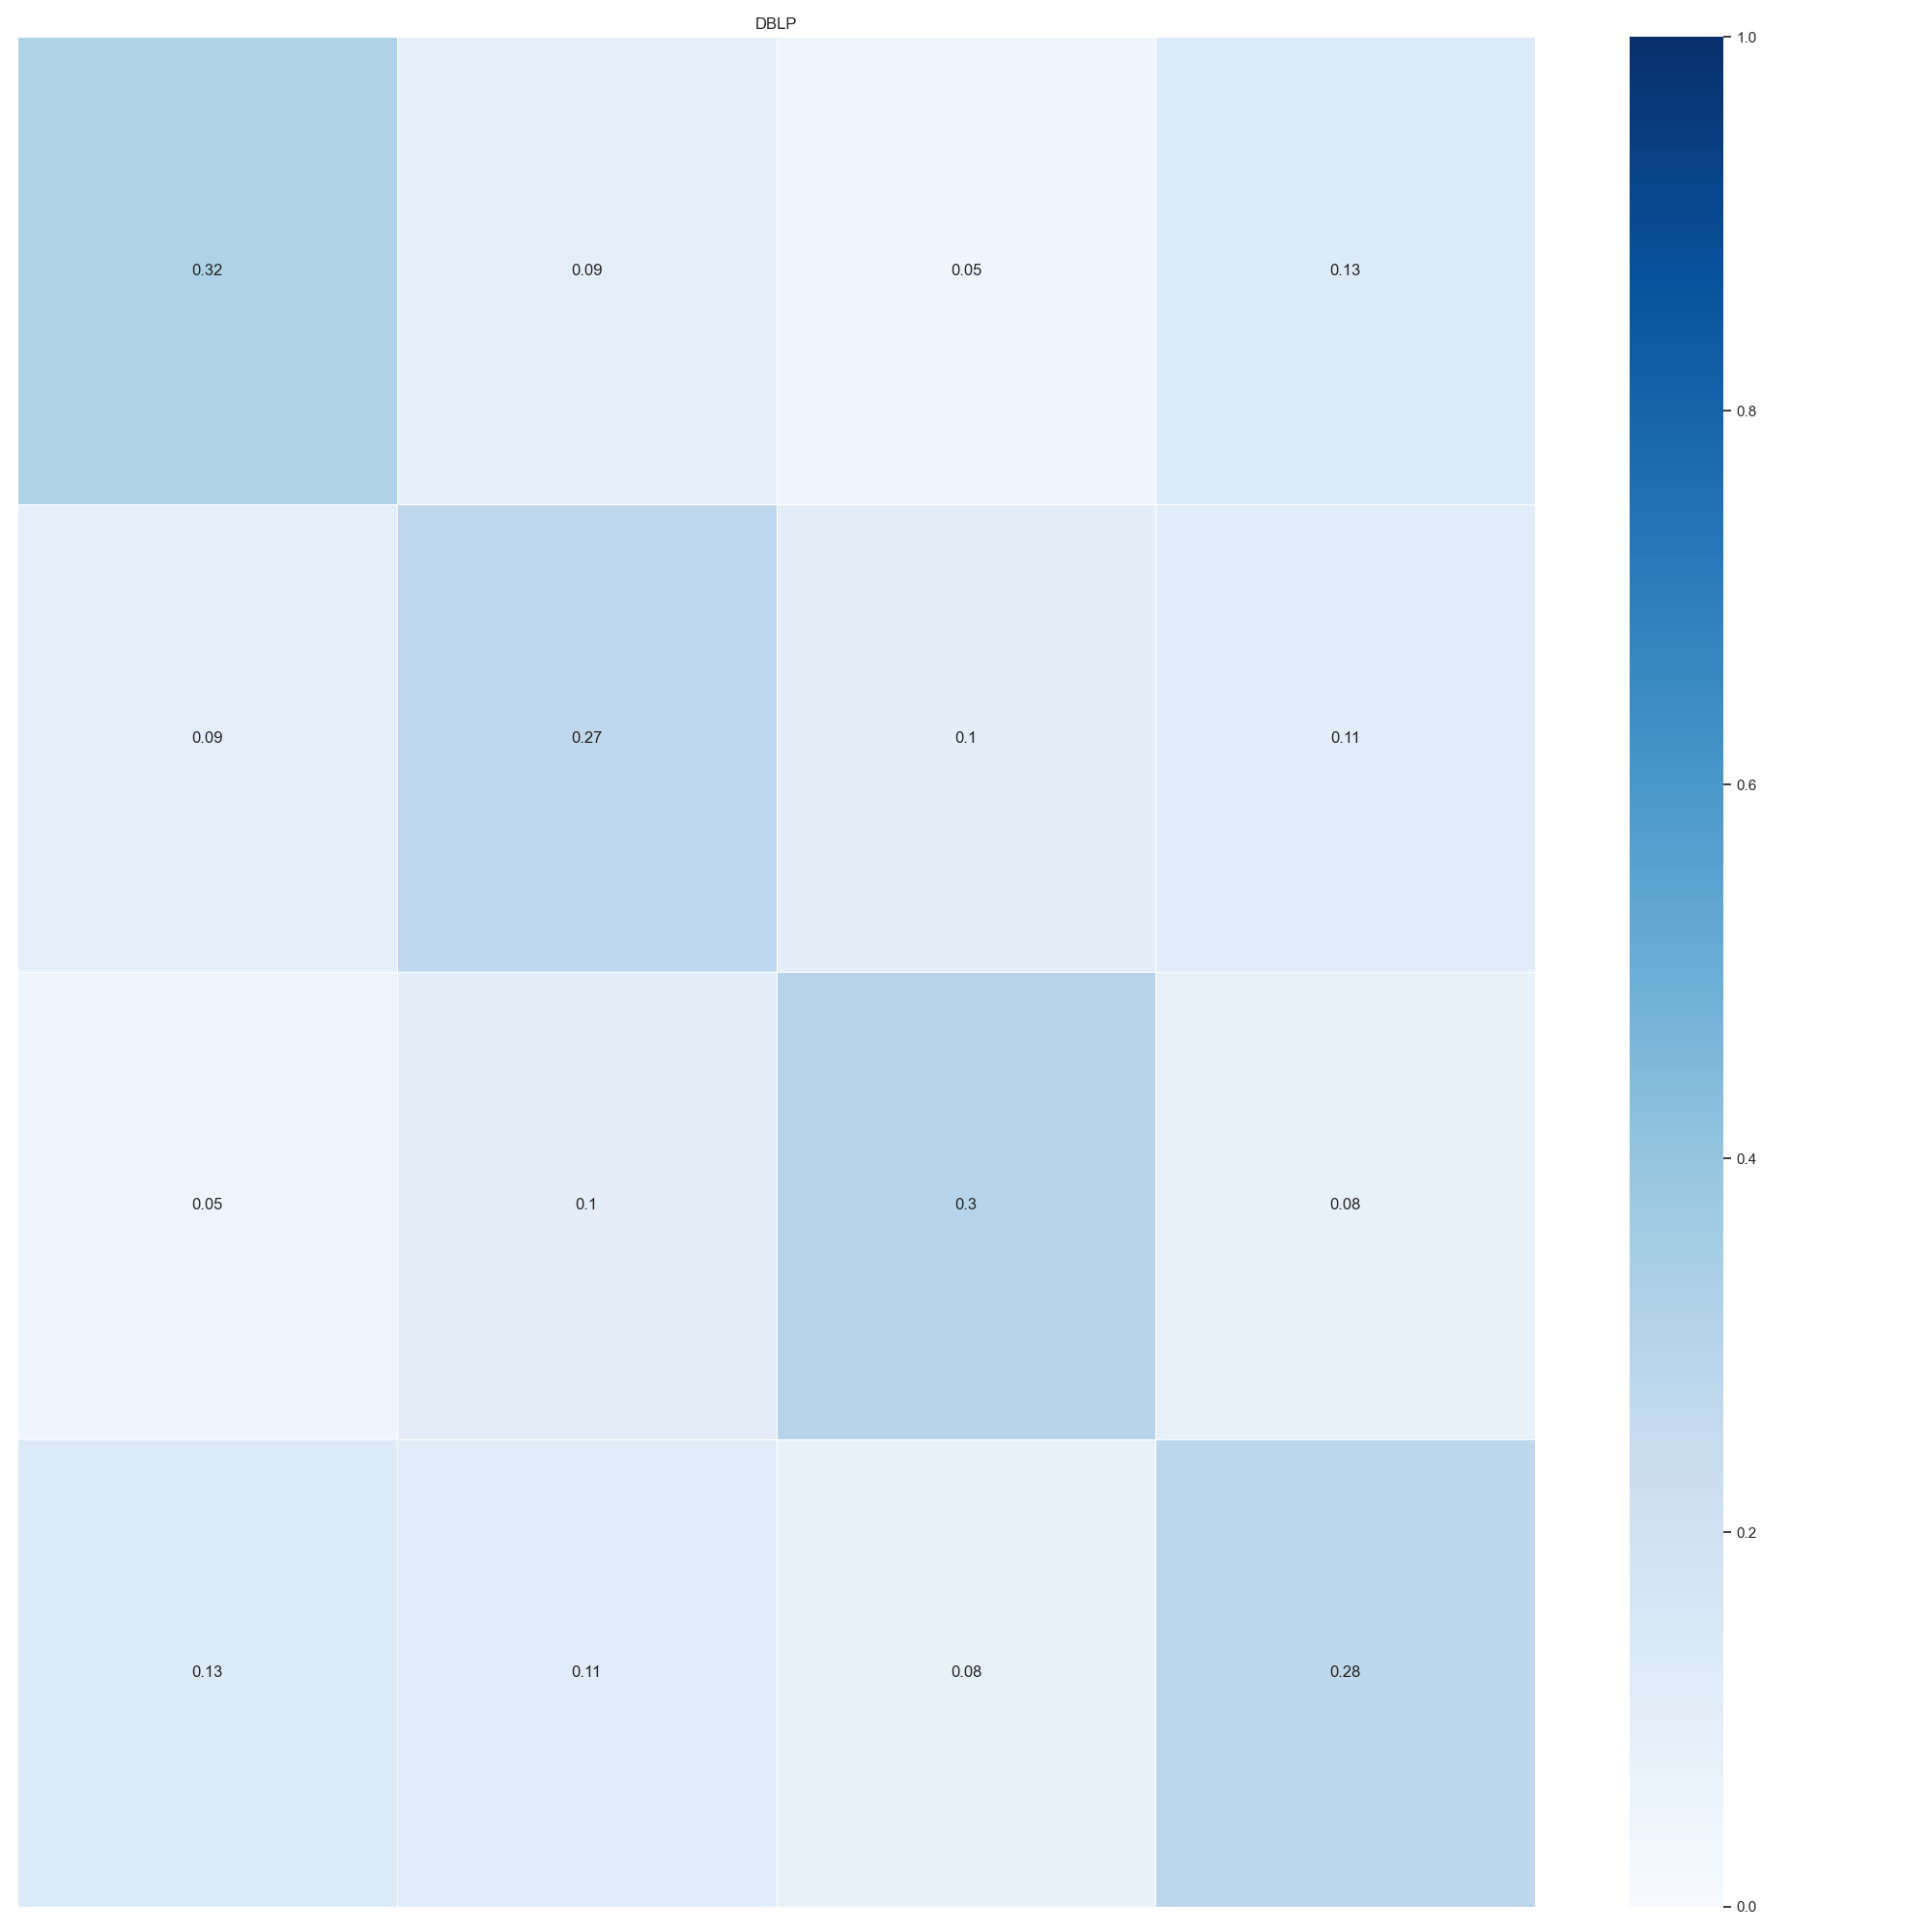}
        \caption{Cross class Neighborhood Similarity in \dblp}
\end{figure}

\begin{figure}
         \centering
       \includegraphics[width=\textwidth]{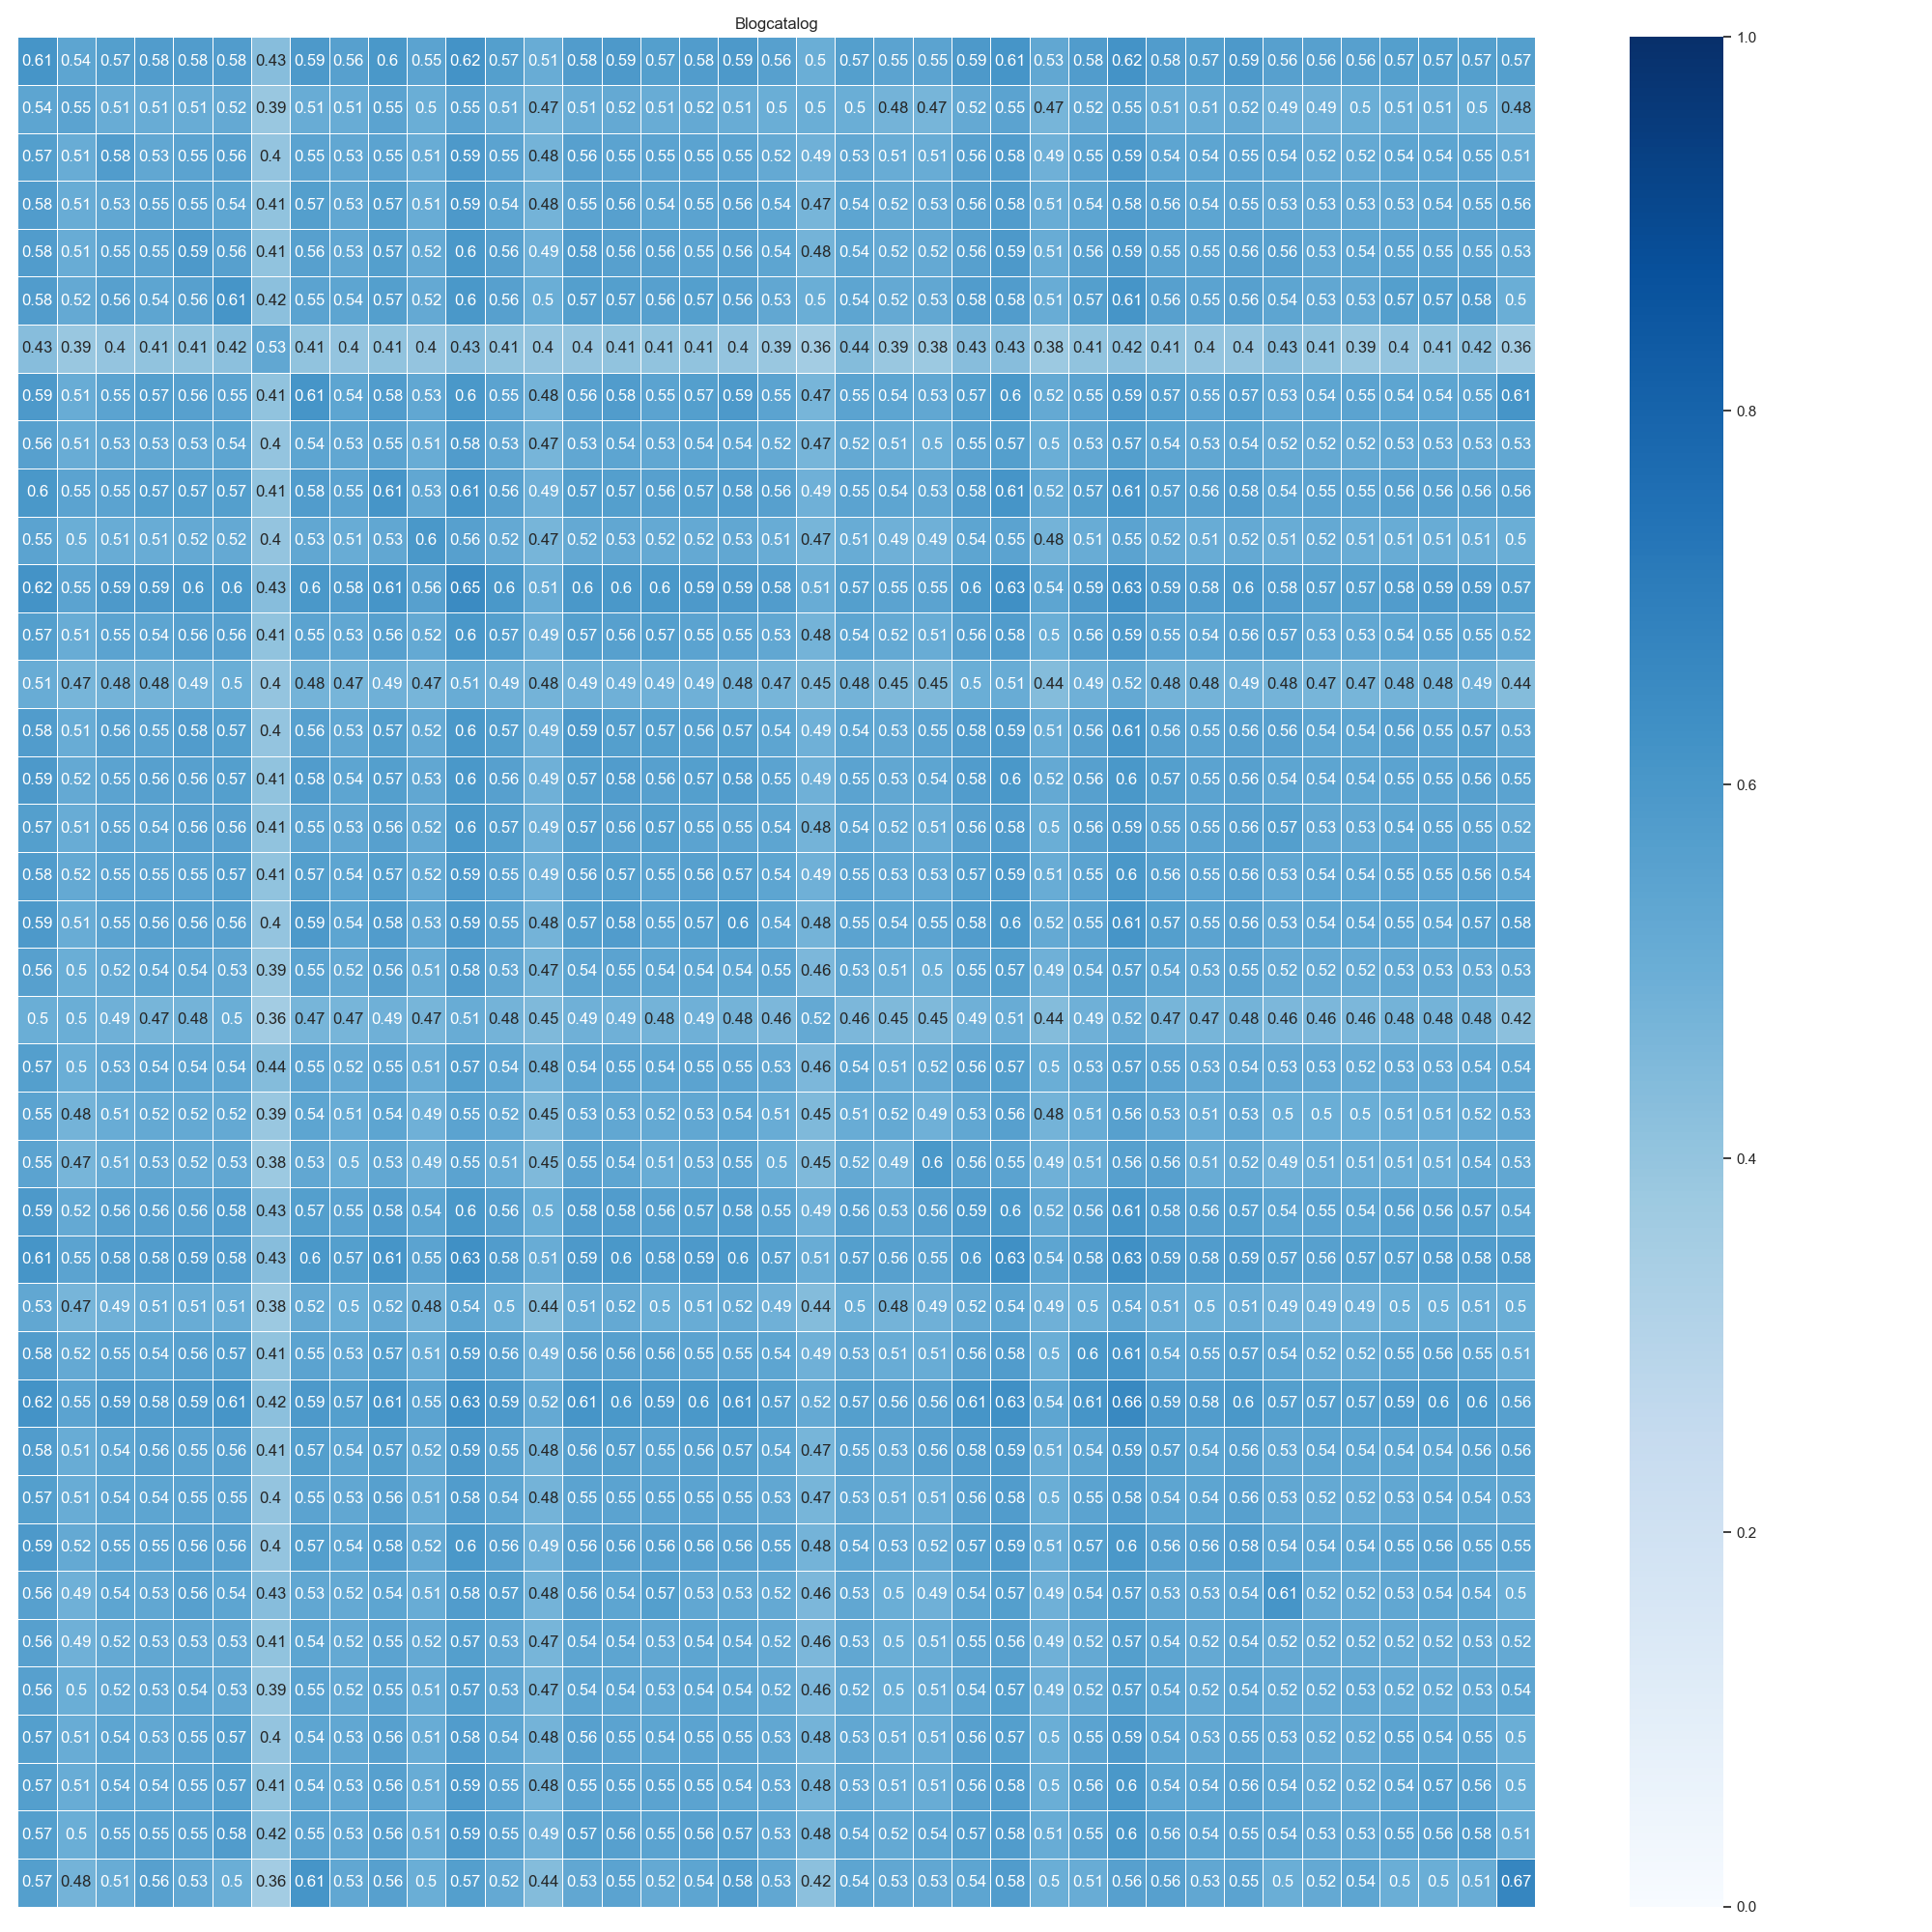}
         \caption{Cross class Neighborhood Similarity in \blog}
     \end{figure}

\begin{figure}
         \centering
         \includegraphics[width=\textwidth]{pcg.png}
         \caption{Cross class Neighborhood Similarity in \pcg}
     \end{figure}

\begin{figure}
         \centering
         \includegraphics[width=\textwidth]{Humloc.png}
         \caption{Cross class Neighborhood Similarity in \humloc}
     \end{figure}

\begin{figure}
         \centering
         \includegraphics[width=\textwidth]{Eukloc.png}
         \caption{Cross class Neighborhood Similarity in \eukloc}
     \end{figure}

\begin{figure}
         \centering
         \includegraphics[width=\textwidth]{homo_0.2.jpg}
         \caption{Cross-class Neighborhood Similarity in graph label homophily=0.2}
         \label{fig:ccns_0.2}
     \end{figure}

\begin{figure}
         \centering
         \includegraphics[width=\textwidth]{homo_0.4.jpg}
         \caption{Cross-class Neighborhood Similarity in graph label homophily=0.4}
     \end{figure}

\begin{figure}
         \centering
         \includegraphics[width=\textwidth]{homo_0.6.jpg}
         \caption{Cross-class Neighborhood Similarity in graph label homophily=0.6}
     \end{figure}

\begin{figure}
         \centering
         \includegraphics[width=\textwidth]{homo_0.8.jpg}
         \caption{Cross-class Neighborhood Similarity in graph label homophily=0.8}
     \end{figure}

\begin{figure}
         \centering
         \includegraphics[width=\textwidth]{homo_1.0.jpg}
         \caption{Cross-class Neighborhood Similarity in graph label homophily=1.0}
     \end{figure}
